# Supplementary material for: Combining Molecular Dynamics and Experimental Methods for the Parametrization of Binary Carbonate-Based Electrolytes
Source: arXiv:2512.13225 ancillary file (2025-12-15)
Supplement: Supplementary file 1 [file supplementary_information.pdf]

# Supporting Information: Combining Molecular Dynamics and Experimental Methods for the Parametrization of Binary Carbonate-Based Electrolytes

Lukas Lehnert, Martin Lorenz, Maria Fernanda Juarez, Max Schammer, Maryam Nojabaee, Monika Schönhoff, Birger Horstmann

## Contents

**S1. Molecular Dynamics** **S1**
- S1.1. Computational Details . . . S1
- S1.2. Particle Numbers . . . S2
- S1.3. Evaluation of the Ion Trajectories . . . S3
- S1.4. Determination of the Scaling Factor . . . S3
- S1.5. Transformation of the Reference Frame . . . S4
- S1.6. Trends in the Diffusion Coefficient . . . S7
- S1.7. Determining the Transport Parameters Using Stefan-Maxwell Diffusivities . . . S8
- S1.8. Radial Distribution Function . . . S8
- S1.9. Electrolyte Viscosity . . . S12
- S1.10. Residence Time and Diffusion Length . . . S14
- S1.11. Ion Association . . . S15
- S1.12. Electrophoretic Mobility . . . S21

**S2. Experiments** **S22**
- S2.1. Experimental Details . . . S22
- S2.2. Concentration Cell Measurements . . . S22
- S2.3. Representative eNMR Phaseshifts . . . S23

# S1. Molecular Dynamics

## S1.1. Computational Details

In the main text, we compute the determine the four parameters of our three electrolytes $LiPF_6$ in EC:EMC, in EC:DMC:PC and in EC:EMC:MP, using MD simulations. This section summarizes the corresponding numerical details. Ringsby et al. compute conductivity values matching strikingly well with experimental data for 1 M $LiPF_6$ in EC:EMC at various temperatures. [1] Therefore, we adapt their simulation set-up for our MD calculations, performed on the high-performance computer cluster bwForCluster JUSTUS 2.

Our MD simulations were run on the Large-scale Atomic/Molecular Massively Parallel Simulator (LAMMPS) [2]. All atom interactions were modelled using the Optimized Potentials for Liquid Simulations (OPLS), [3] where the required force field parameters and partial charges for the solvent molecules, $Li^+$ and $PF_6^-$ ions were taken from Maestro (Schrödinger) [4], Jensen et al. [5] and Lopes et al. [6] However, the employed non-polarizable OPLS force field neglects the solvent screening effects due to solvent polarization and therefore, likely overestimates the effective charges of the ions. This could lead to increased ion associations and thus, decreased ionic conductivities compared to experimental values. [1] Introducing a screening factor $\zeta$ lowering the effective charges of the ions yields more consistent simulation results. [1,7] Here, we optimized our MD simulations by adjusting $\zeta$ for our electrolytes at $c = 1.0\,\mathrm{M}$ and various temperatures (see SI Table S3).

Our simulated particle ensembles consisted of 500–1000 solvent molecules and varying ion numbers depending on the desired salt concentration (see SI Table S1).

The starting configuration of each ensemble was generated by the PACKMOL package, distributing the particles randomly in a cubic simulation box with periodic boundary conditions. [8] After minimizing the energy of the package, the particles were initialized with random starting velocities corresponding to a temperature of $T = 25\,^\circ\mathrm{C}$ and were equilibrated for 3 ns under isothermal-isobaric constraints (npt-ensemble) at a pressure of $p = 1\,\mathrm{atm}$. During the subsequent 3 ns, the ensemble cooled down to the desired target temperature, followed by another 3.5 ns long equilibration process. Ringsby et al. have previously shown, that the

applied cooling rate is sufficiently slow.[1] Averaging the electrolyte volume over the last 0.5 ns defined the fixed box volume of the final canonical production run (nvt-ensemble). In this run, long simulation durations of 50–170 ns ensured, that Fickian diffusion processes established.

During the npt- and nvt-ensemble simulations, the Nose-Hoover thermostat and barostat regulated the temperature and the pressure with damping factors of 100 fs and 1000 fs respectively.[9–12] While the velocity-Verlet algorithm solved the equations of motion with a 1 fs time step,[13] the pppm solver ($10^{-5}$ accuracy) calculated the long-range Coulombic interactions in reciprocal space.[14] Short-range Coulombic and 12–6 Lennard-Jones interactions with a 14 Å cut-off distance were directly quantified. For determining the corresponding Lennard-Jones parameters between different atom types, the geometric mixing rule was applied.

The last 40–160 ns of the production run were subject to the evaluation process (see SI Section S1.3). To calculate the Onsager transport coefficients from the ion trajectories (see Eq. 3) we adapted the code provided by Fong et al.[15,16], which utilizes the MDAnalysis package (Python)[17,18]. The averaged results of three MD simulations yielded the transport parameters and the corresponding standard deviation for the electrolytes at one specific concentration and temperature pair.

## S1.2. Particle Numbers

The particle ensembles modeled in our MD simulations comprise 500 solvent molecules for each of our electrolytes $LiPF_6$ in EC:EMC, in EC:DMC:PC and in EC:EMC:MP. In order to determine the specific particle numbers of the corresponding electrolyte components, we translate the volume ratios into mass ratios using the respective solvent densities stated by the manufacturers (see SI Table S2). Combining the mass ratios with the mole masses of the molecules yields the desired particle numbers.

**Table S2.** Densities of the individual electrolyte components[19].

| Component | Density (g/ml) |
|---|---|
| EC | 1.321 |
| EMC | 1.006 |
| DMC | 1.069 |
| PC | 1.204 |
| MP | 0.915 |

Adding $Li^+$ and $PF_6^-$ ions to the solvent blends increases the salt concentration. In order to find the right number of ions for our target concentrations, we conduct multiple MD simulations at 20 °C with varying ion numbers. Table S1 shows the most consistent particle numbers with the desired concentrations. Since the ion numbers would be tiny for the lowest concentration, we double the total number of particles in these ensembles.

**Table S1.** Particle numbers used in our MD simulations.

| Electrolyte | $c$ (M) | $Li^+$ | $PF_6^-$ | EC | EMC | DMC | PC | MP |
|---|---|---|---|---|---|---|---|---|
| $LiPF_6$ in EC:EMC (3:7, weight) | 0.1 | 9 | 9 | 336 | 664 | - | - | - |
| | 0.5 | 23 | 23 | 168 | 332 | - | - | - |
| | 1.0 | 47* | 47* | 168* | 332* | - | - | - |
| | 1.5 | 74 | 74 | 168 | 332 | - | - | - |
| | 2.0 | 103 | 103 | 168 | 332 | - | - | - |
| | 2.5 | 134 | 134 | 168 | 332 | - | - | - |
| | 3.0 | 168 | 168 | 168 | 332 | - | - | - |
| $LiPF_6$ in EC:DMC:PC (27:63:10, volume) | 0.1 | 8 | 8 | 320 | - | 588 | 92 | - |
| | 0.5 | 20 | 20 | 160 | - | 294 | 46 | - |
| | 1.0 | 42 | 42 | 160 | - | 294 | 46 | - |
| | 1.5 | 65 | 65 | 160 | - | 294 | 46 | - |
| | 2.0 | 90 | 90 | 160 | - | 294 | 46 | - |
| | 2.5 | 117 | 117 | 160 | - | 294 | 46 | - |
| | 3.0 | 146 | 146 | 160 | - | 294 | 46 | - |
| $LiPF_6$ in EC:EMC:MP (2:6:2, volume) | 0.1 | 9 | 9 | 276 | 534 | - | - | 190 |
| | 0.5 | 23 | 23 | 138 | 267 | - | - | 95 |
| | 1.0 | 48 | 48 | 138 | 267 | - | - | 95 |
| | 1.5 | 75 | 75 | 138 | 267 | - | - | 95 |
| | 2.0 | 104 | 104 | 138 | 267 | - | - | 95 |
| | 2.5 | 135 | 135 | 138 | 267 | - | - | 95 |
| | 3.0 | 170 | 170 | 138 | 267 | - | - | 95 |

*Taken from Ringsby et al.[1]

The particle numbers for 1 M $LiPF_6$ in EC:EMC were taken from Ringsby et al.[1]. Note that the ion concentration is insensitive to changes in the scaling factor $\zeta$ within the range examined in this work (see SI Section S1.4).

## S1.3. Evaluation of the Ion Trajectories

The trajectories of the $Li^+$ and $PF_6^-$ ions in our MD simulations reveal the Onsager transport coefficients $L^{++}$, $L^{--}$ and $L^{+-}$ by applying equation 3. Evaluating the equation requires equilibrated trajectories and long simulation durations such that Fickian diffusion processes establish.[1,20] In the Fickian regime, the bracketed term in equation 3 (which is often denoted as mean square displacement $MSD$) scales linear over time, i.e. it is proportional to $t^\beta$ where $\beta = 1$. Therefore, calculating $\beta(t)$ with

$$\beta(t) = \frac{d \ln MSD}{d \ln t} \tag{S1}$$

allows for identifying the linear segment of $MSD$.
In order to evaluate our MD simulations, we calculate the corresponding $MSD$s using an adapted version of the code provided by Fong et al.[15,16] We apply a Savitzky-Golay filter[21] on $\beta(t)$ and linearly fit $MSD$ for the time interval where $|1 - \beta^{\text{filtered}}(t)|$ is small. Figure S1 shows an exemplary evaluation of the $MSD$ data needed for calculating $L^{++}$ of 1 M $LiPF_6$ in EC:EMC:MP at 20 °C.
For some MD simulations, the correlation between anions and cations is very weak, making the identification of the linear regime of the corresponding $MSD$ difficult. In order to determine $L^{+-}$, we therefore calculate $\kappa$ and $t_+$ with

$$\kappa = \frac{F^2}{6k_\mathrm{B}TV} \lim_{t\to\infty} \frac{\mathrm{d}}{\mathrm{d}t} \left\langle \sum_i \sum_j z_i z_j \cdot \sum_\alpha \left[\boldsymbol{r}_i^\alpha(t) - \boldsymbol{r}_i^\alpha(0)\right] \cdot \sum_\beta \left[\boldsymbol{r}_j^\beta(t) - \boldsymbol{r}_j^\beta(0)\right] \right\rangle \tag{S2}$$

and

$$t_+ = \frac{F^2}{6k_\mathrm{B}TV\kappa} \lim_{t\to\infty} \frac{\mathrm{d}}{\mathrm{d}t} \left\langle \sum_j z_+ z_j \cdot \sum_\alpha \left[\boldsymbol{r}_+^\alpha(t) - \boldsymbol{r}_+^\alpha(0)\right] \cdot \sum_\beta \left[\boldsymbol{r}_j^\beta(t) - \boldsymbol{r}_j^\beta(0)\right] \right\rangle \tag{S3}$$

and combine them with the outcomes of $L^{++}$ and $L^{--}$ using equations 4 and 5. Solving both equations for $L^{+-}$ and averaging the results yields the desired quantity.

## S1.4. Determination of the Scaling Factor

Using unpolarized force fields for the MD simulations omits solvent screening effects due to solvent polarization, lowering the effective charges of the ions. The

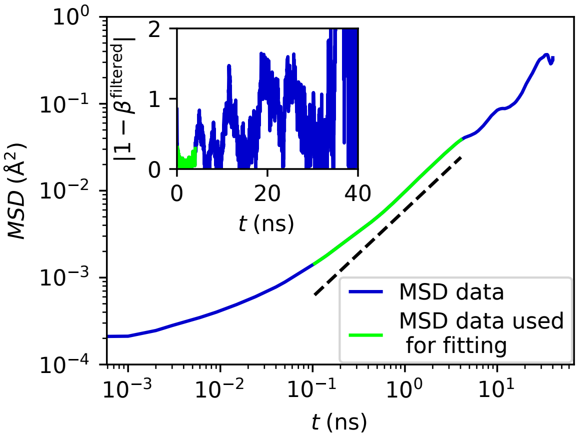


**Figure S1.** Exemplary $MSD$ data of 1 M $LiPF_6$ in EC:EMC:MP at 20 °C. The green data highlights the linear regime of $MSD$, used for evaluating $L^{++}$. For comparison purposes, the dashed line indicates ideal linear behavior. The inset shows the absolute deviation of $\beta(t)$ (see SI Eq. S1) from 1. Small values imply linear $MSD$ behavior.

**Table S3.** Optimized scaling factor $\zeta$ for the effective charges of the $Li^+$ and $PF_6^-$ ions.

| Electrolyte | $\zeta$ |
|---|---|
| $LiPF_6$ in EC:EMC (3:7, weight) | 0.75 |
| $LiPF_6$ in EC:DMC:PC (27:63:10, volume) | 0.75 |
| $LiPF_6$ in EC:EMC:MP (2:6:2, volume) | 0.73 |

less screened ions are more likely to form ion clusters leading to decreased conductivities $\kappa$.[1] To compensate this effect, a scaling factor $\zeta$ can be introduced, reducing the effective charges of the ions.[1,7] This enables obtaining more consistent simulation results compared to experimental conductivity data.
Here, we optimize $\zeta$ for each of our electrolytes $LiPF_6$ in EC:EMC, in EC:DMC:PC and in EC:EMC:MP. For this, we calculate the corresponding conductivities at a concentration of $c = 1.0$ M at various temperatures $-20\,°\mathrm{C} \leq T \leq 20\,°\mathrm{C}$ with different scaling factors $0.7 < \zeta \leq 0.8$ and compare the results to experimental data.[1,22] Assuming a linear dependence of the modeled conductivities on the scaling factor allows for estimating an optimal $\zeta(T)$ value for each temperature. The average of the optimal values yields the final scaling factor $\zeta$ used for the MD simulations. Note that this method results in one scaling factor for all temperatures and thus omits any temperature dependent solvent screening effects.[23,24] Since we determine $\zeta$ for only $c = 1.0$ M, we also neglect any concentration dependence of this quantity. Table S3 lists the optimized scaling factors for the three electrolytes. Note that we optimize $\zeta$ for $LiPF_6$ in EC:EMC using the measurement results of Ringsby et al.[1] This leads to the slight deviations between the simulated conductivities and the experimental data of Landesfeind et al.[25], evident in Figure 1.
Figure S2 exemplary shows the optimization process

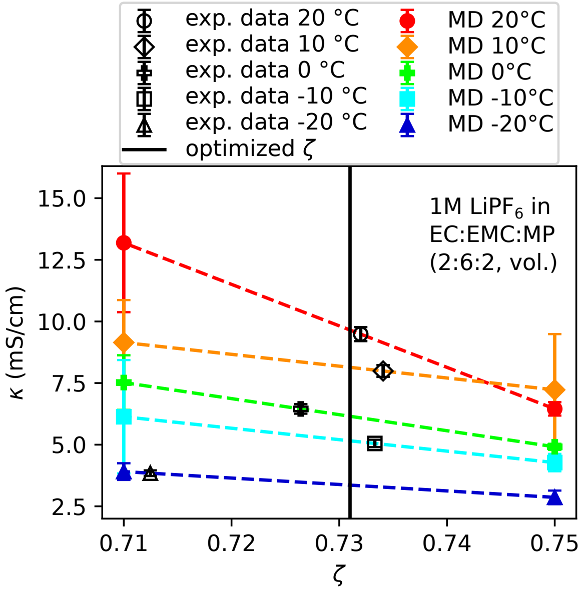


**Figure S2.** Exemplary optimization process of the scaling factor $\zeta$ for 1 M $LiPF_6$ in EC:EMC:MP.

for the EC:EMC:MP electrolyte. Each calculated data point comprises the average of three MD simulation runs.

## S1.5. Transformation of the Reference Frame

In our concentrated solution theory[26–28], the electrolyte parameters are dependent on the considered reference frame $\Psi$. In order to compare parameters determined in different reference frames $\Psi$ and $\tilde{\Psi}$, we have to transform them into a common frame.
Schammer[29] derives in his work the transformation for the Onsager transport coefficients $\boldsymbol{L}$, assuming negligibly small viscous forces,

$$\boldsymbol{L}^{\Psi} = \boldsymbol{U}^{\tilde{\Psi}\Psi} \boldsymbol{L}^{\tilde{\Psi}} \left(\boldsymbol{U}^{\tilde{\Psi}\Psi}\right)^{T}. \tag{S4}$$

The transformation matrix $\boldsymbol{U}^{\tilde{\Psi}\Psi}$ is defined by

$$U^{\tilde{\Psi}\Psi}_{\alpha\beta} = \delta_{\alpha\beta} + \tilde{\Psi}_{\beta}\frac{c_\alpha}{c_\beta}\left(\frac{\Psi_0}{\tilde{\Psi}_0} - \frac{\Psi_\beta}{\tilde{\Psi}_\beta}\right), \tag{S5}$$

where in our case, the subscript 0 corresponds to the solvent and the subscripts $\alpha, \beta$ correspond to the $Li^+$ and $PF_6^-$ ions. For our electro-neutral, three component electrolyte, this results with $c = c_+ = c_-$, $z_0 = 0$, $z_+ = -z_- = 1$ and $\sum_i^n \Psi_i = 1$ in the transformation rules for the transport parameters,

$$\kappa^{\Psi} = \kappa^{\tilde{\Psi}}, \tag{S6}$$

$$t_+^{\Psi} = \frac{\Psi_0}{\tilde{\Psi}_0} t_+^{\tilde{\Psi}} - \tilde{\Psi}_- \left(\frac{\Psi_0}{\tilde{\Psi}_0} - \frac{\Psi_-}{\tilde{\Psi}_-}\right), \tag{S7}$$

$$\frac{D_\pm^{\Psi}}{TDF^{\Psi}} = \left(\frac{\Psi_0}{\tilde{\Psi}_0}\right)^2 \frac{D_\pm^{\tilde{\Psi}}}{TDF^{\tilde{\Psi}}}. \tag{S8}$$

According to our approach, the Onsager coefficients express the independent fluxes via the frame-dependent chemical driving forces of the $Li^+$ ions,[28]

$$\nabla\mu^{\Psi} = \nabla\mu_+ + \nabla\mu_- - \frac{c_0}{c}\frac{\Psi_+ + \Psi_-}{\Psi_0}\nabla\mu_0 \tag{S9a}$$

$$= \frac{RT}{c}\left[1 + \frac{\partial \ln\left(f_\pm^{\Psi}\right)}{\partial \ln\left(c\right)}\right]\nabla c. \tag{S9b}$$

Using the Gibbs-Duhem relation $\sum_i^n c_i \nabla\mu_i = 0$ in Eq. S9a yields

$$\nabla\mu^{\Psi} = -\frac{c_0}{c\Psi_0}\nabla\mu_0. \tag{S10}$$

The comparison of Eq. S10 to Eq. S9b reveals the transformation rule for the thermodynamic factor $TDF^{\Psi} = 1 + \frac{\partial \ln(f_\pm^{\Psi})}{\partial \ln(c)}$

$$TDF^{\Psi} = \frac{\Psi_0}{\tilde{\Psi}_0} TDF^{\tilde{\Psi}}. \tag{S11}$$

Table S4 lists the coefficients $\Psi_i$ for the center-of-mass velocity frame (COM), the solvent velocity frame (SOL) and the volume-based frame (VOL) required for the transformations. While the mass fractions $\omega_i$ are easily accessible from our MD simulations, the partial molar volumes $\nu_i$ are unknown. In order to calculate $\nu_i$, we use the experimental partial molar volume of the $LiPF_6$ salt in EC:DEC (1:1, weight) at $T = 25\,°C$[30] and the radius of the $Li^+$ ion[31].

**Table S4.** Coefficients $\Psi_i$ for the individual reference frames.

| Frame | $\Psi_i$ |
|---|---|
| COM | $\omega_i$ |
| SOL | $\delta_{0i}$ |
| VOL | $c_i\nu_i$ |

In the main text of this work, we present the electrolyte parameters in the VOL frame. However, the literature determines these parameters often in different reference frames. Therefore, we present our findings in the COM and SOL frame as well (see SI Figures S3 and S4). For comparison, we additionally transform the transference numbers obtained from the eNMR measurements into these frames employing the same coefficients $\Psi_i$ as used for the frame transformation of our MD simulation results.
In order to fit the transformed parameters, we use the same procedure as in the main text, except for $t_+$. The transformation of $t_+^{VOL}$ into $t_+^{COM}$ and $t_+^{SOL}$ introduces a concentration dependence, which we fit linearly,

$$t_+ = t_0 + t_1 c. \tag{S12}$$

Tables S5 and S6 list the corresponding fitting coefficients for all electrolyte parameters.
Ringsby et al. have calculated the transference number $t_+^{SOL}$ at $c = 1.0\,M$ for $LiPF_6$ in EC:EMC, using MD simulations with a scaling factor of $\zeta = 0.8$ at slightly different temperatures. As Figure S4 shows, their data matches our MD simulations fairly well.

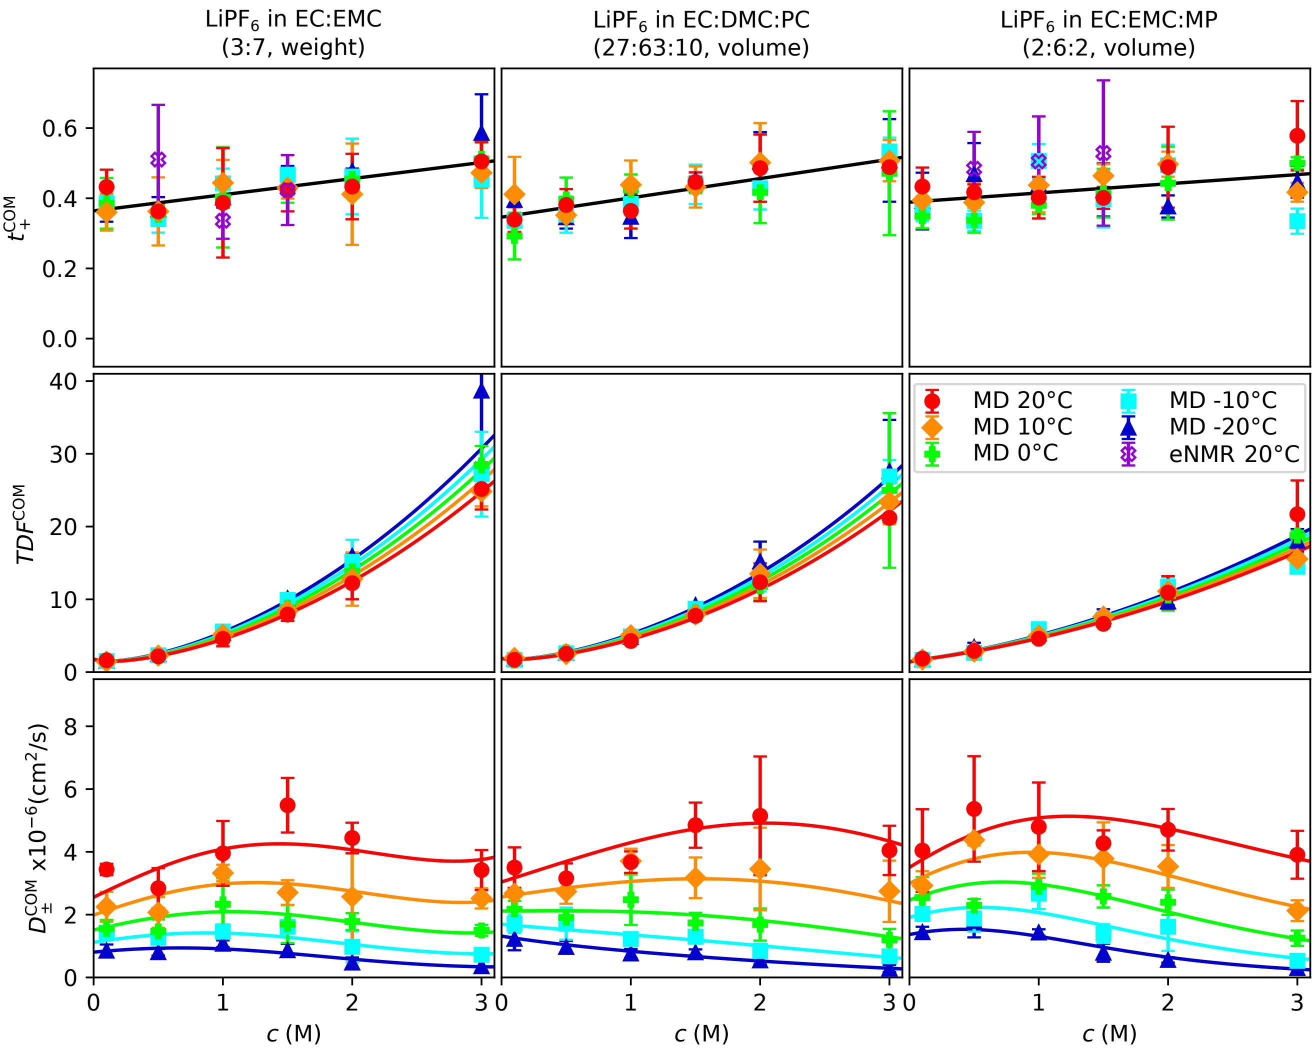


**Figure S3.** Electrolyte parameters obtained by our MD simulations together with their corresponding fit functions in the COM frame.

**Table S5.** Fit coefficients $t_i$ (in $\mathrm{M}^{-i}$), $T_0$ (in K), $a_{ij}$ (in $\mathrm{M}^{-i/2}\,\mathrm{K}^{-j}$), $T_{gi}$ (in $\mathrm{K\,M}^{-i}$) and $D_{ij}$ (in $\mathrm{K}^j\,\mathrm{M}^{-i}$) for the electrolyte parameters in the COM frame.

| Electrolyte parameter | Fit coefficient | $LiPF_6$ in EC:EMC (3:7, weight) | $LiPF_6$ in EC:DMC:PC (27:63:10, volume) | $LiPF_6$ in EC:EMC:MP (2:6:2, volume) |
|---|---|---|---|---|
| $t_+^{COM}$ | $t_0$ | 0.364 | 0.346 | 0.389 |
| | $t_1$ | 0.046 | 0.055 | 0.026 |
| $a^{COM}(c,T)$ | $T_0$ | 293.15 | 293.15 | 293.15 |
| | $a_{00}$ | $1.150 \cdot 10^0$ | $1.245 \cdot 10^0$ | $8.407 \cdot 10^{-1}$ |
| | $a_{10}$ | $-9.519 \cdot 10^{-1}$ | $-5.961 \cdot 10^{-1}$ | $5.235 \cdot 10^{-1}$ |
| | $a_{30}$ | $2.470 \cdot 10^0$ | $2.044 \cdot 10^0$ | $1.357 \cdot 10^0$ |
| | $a_{31}$ | $-5.776 \cdot 10^{-3}$ | $-5.322 \cdot 10^{-3}$ | $-4.240 \cdot 10^{-3}$ |
| $D_\pm^{COM}$ | $T_{g0}$ | $4.993 \cdot 10^1$ | $1.212 \cdot 10^2$ | $1.930 \cdot 10^2$ |
| | $T_{g1}$ | $3.961 \cdot 10^1$ | $-1.369 \cdot 10^1$ | $-1.648 \cdot 10^1$ |
| | $D_{00}$ | $-3.048 \cdot 10^0$ | $-4.317 \cdot 10^0$ | $-4.841 \cdot 10^0$ |
| | $D_{01}$ | $-6.189 \cdot 10^2$ | $-2.064 \cdot 10^2$ | $-6.148 \cdot 10^1$ |
| | $D_{10}$ | $5.270 \cdot 10^{-1}$ | $1.640 \cdot 10^0$ | $5.834 \cdot 10^{-1}$ |
| | $D_{11}$ | $5.488 \cdot 10^1$ | $-2.664 \cdot 10^2$ | $-3.661 \cdot 10^1$ |
| | $D_{20}$ | $-1.957 \cdot 10^{-1}$ | $-9.987 \cdot 10^{-2}$ | $9.150 \cdot 10^{-2}$ |
| | $D_{21}$ | $2.011 \cdot 10^1$ | $-8.245 \cdot 10^0$ | $-3.337 \cdot 10^1$ |

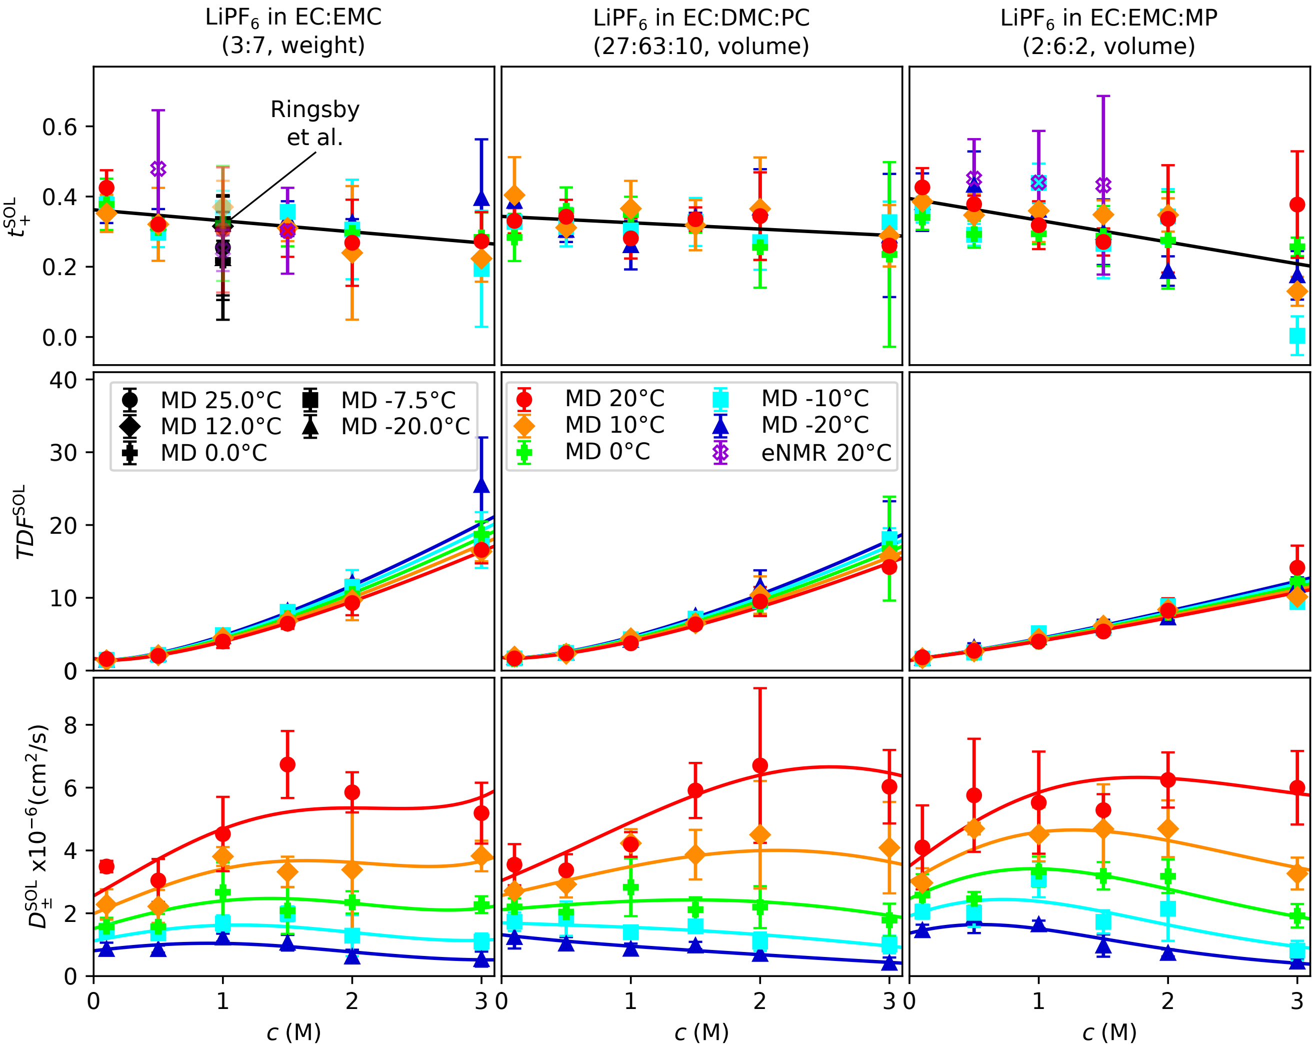


**Figure S4.** Electrolyte parameters obtained by our MD simulations together with their corresponding fit functions in the SOL frame. The black data points show the MD simulations of Ringsby et al.,[1] using $\zeta = 0.8$.

**Table S6.** Fit coefficients $t_i$ (in $M^{-i}$), $T_0$ (in K), $a_{ij}$ (in $M^{-i/2}\,K^{-j}$), $T_{gi}$ (in $K\,M^{-i}$) and $D_{ij}$ (in $K^j\,M^{-i}$) for the electrolyte parameters in the SOL frame.

| Electrolyte parameter | Fit coefficient | $LiPF_6$ in EC:EMC (3:7, weight) | $LiPF_6$ in EC:DMC:PC (27:63:10, volume) | $LiPF_6$ in EC:EMC:MP (2:6:2, volume) |
|---|---|---|---|---|
| $t_+^{SOL}$ | $t_0$ | 0.362 | 0.343 | 0.394 |
| | $t_1$ | $-0.031$ | $-0.018$ | $-0.062$ |
| $a^{SOL}(c,T)$ | $T_0$ | 293.15 | 293.15* | 293.15 |
| | $a_{00}$ | $1.082 \cdot 10^0$ | $1.195 \cdot 10^0$ | $8.127 \cdot 10^{-1}$ |
| | $a_{10}$ | $-7.703 \cdot 10^{-1}$ | $-4.623 \cdot 10^{-1}$ | $5.995 \cdot 10^{-1}$ |
| | $a_{30}$ | $2.353 \cdot 10^0$ | $1.948 \cdot 10^0$ | $1.281 \cdot 10^0$ |
| | $a_{31}$ | $-5.788 \cdot 10^{-3}$ | $-5.408 \cdot 10^{-3}$ | $-4.598 \cdot 10^{-3}$ |
| $D_\pm^{SOL}$ | $T_{g0}$ | $5.009 \cdot 10^1$ | $1.212 \cdot 10^2$ | $1.930 \cdot 10^2$ |
| | $T_{g1}$ | $3.950 \cdot 10^1$ | $-1.369 \cdot 10^1$ | $-1.649 \cdot 10^1$ |
| | $D_{00}$ | $-3.050 \cdot 10^0$ | $-4.317 \cdot 10^0$ | $-4.841 \cdot 10^0$ |
| | $D_{01}$ | $-6.180 \cdot 10^2$ | $-2.063 \cdot 10^2$ | $-6.149 \cdot 10^1$ |
| | $D_{10}$ | $5.862 \cdot 10^{-1}$ | $1.696 \cdot 10^0$ | $6.438 \cdot 10^{-1}$ |
| | $D_{11}$ | $5.412 \cdot 10^1$ | $-2.662 \cdot 10^2$ | $-3.661 \cdot 10^1$ |
| | $D_{20}$ | $-1.945 \cdot 10^{-1}$ | $-9.936 \cdot 10^{-2}$ | $9.206 \cdot 10^{-2}$ |
| | $D_{21}$ | $2.015 \cdot 10^1$ | $-8.260 \cdot 10^0$ | $-3.339 \cdot 10^1$ |

## S1.6. Trends in the Diffusion Coefficient

In this section, we aim to deepen the physical understanding of the diffusion coefficient trends observed in our simulations. For this, we analyze two multiplicative contributions to the diffusion coefficient $D_{\pm}^{\mathrm{VOL}} = f_{\mathrm{O}}\, TDF$ (see Eq. 6), using $LiPF_6$ in EC:EMC as an example. The results are subsequently compared to the solid polymer electrolyte LiTFSI in PEO at 90 °C.[32]

The first factor $f_{\mathrm{O}} = \frac{-z_+z_-\left(L^{++}L^{--}-L^{+-2}\right)}{z_+^2L^{++}+2z_+z_-L^{+-}+z_-^2L^{--}}\frac{RT}{c}$ describes the diffusion coefficient with respect to thermodynamic driving force multiplied by an energy density contribution, which originates from the chemical potential gradient. $f_{\mathrm{O}}$ contains a combination of independent Onsager transport coefficients, which capture the motion correlations of the ions. The second factor $TDF$ denotes the thermodynamic factor, closely related to the molar-based salt activity $f_{\pm}$.

For our carbonate-based electrolyte, both factors can easily be calculated from MD simulation data. For the PEO electrolyte, Gao et al. provide fit functions for the diffusion coefficient and the thermodynamic factor, which depends on the molal activity coefficient $\gamma_{\pm}$.[32] To compare the data to our results, we determine the molar-based thermodynamic factor from their data and calculate $f_{\mathrm{O}} = \frac{D_{\pm}}{TDF}$. The results of both electrolytes are shown in Figure S5, where we normalize each factor by its individual value at $c = 1.0\,\mathrm{M}$.

For our carbonate-based electrolyte, $f_{\mathrm{O}}$ shows monotonically decreasing behavior with increasing salt concentration $c$. Therefore, this factor suggests decreasing diffusion coefficients. The observed trend originates in the individual Onsager transport coefficients, which capture the motion correlation between the ions. The coefficients $L^{++}$ and $L^{--}$ consist of two additive terms $L^{ii} = L^{ii}_{\mathrm{distinct}} + L^{ii}_{\mathrm{self}}$. These account for the correlations between particles of the same species and the ideal Nernst-Einstein transport contributions, respectively (see SI Eqs. S19 and S20). Additionally, $L^{+-}$ captures the motion correlation between the two ionic species. Figure S6 compares the transport coefficients and reveals that $f_{\mathrm{O}}$ is dominated by the $L^{ii}_{\mathrm{self}}$ terms.

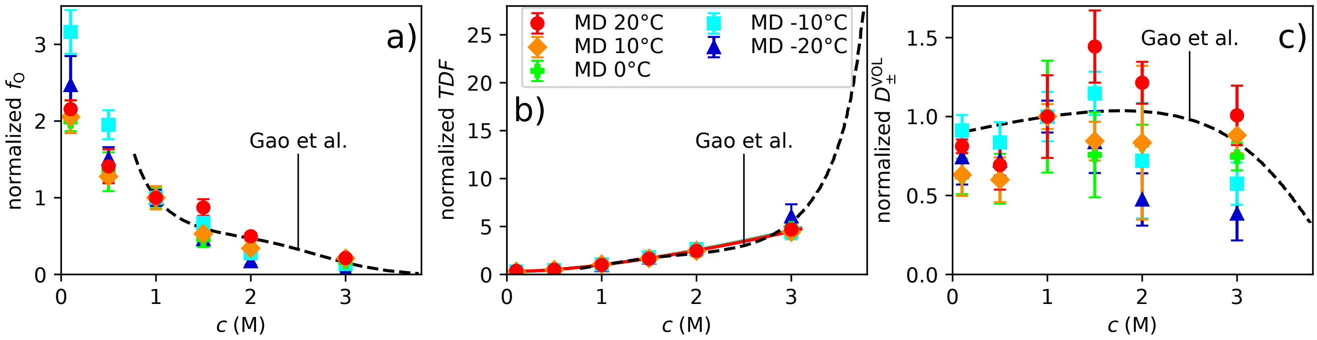


**Figure S5.** a) Factor $f_{\mathrm{O}}$, b) thermodynamic factor $TDF$ , and c) the diffusion coefficient $D_{\pm}^{\mathrm{VOL}}$ in the VOL frame, each normalized at $c = 1.0\,\mathrm{M}$ for each temperature. The data of $LiPF_6$ in EC:EMC (colored data) were calculated from our MD simulations. The data of the PEO electrolyte (dashed lines) were taken from Gao et al.[32]

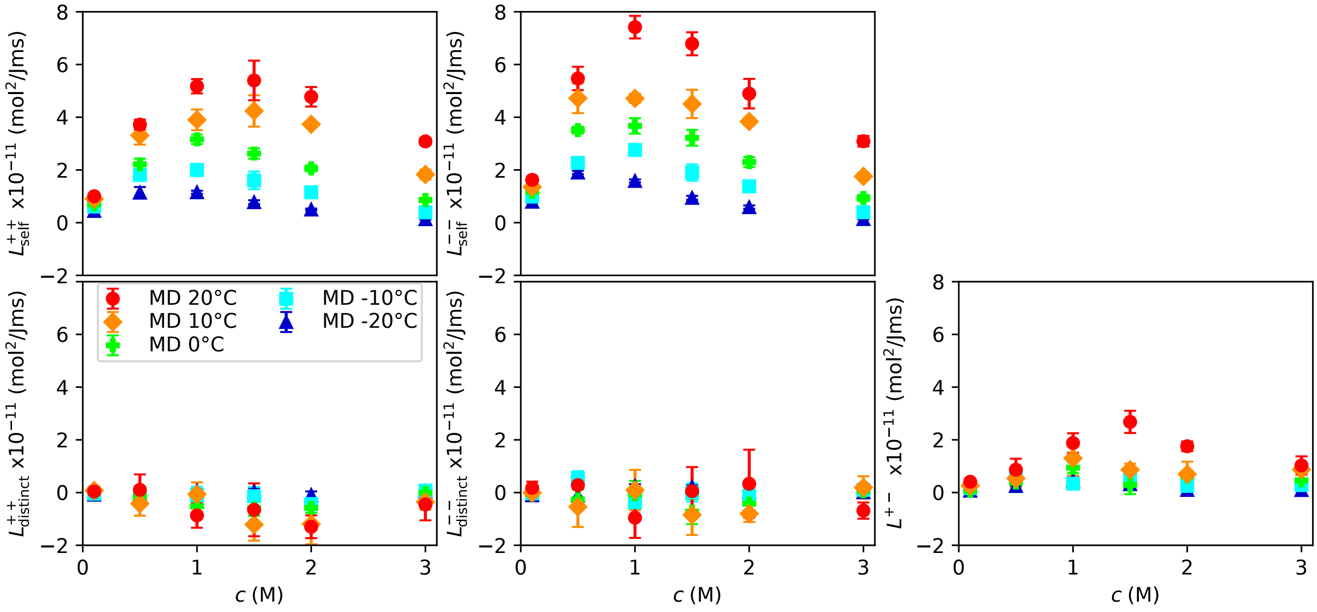


**Figure S6.** Onsager transport coefficients of $LiPF_6$ in EC:EMC in the COM frame.

These quantities are closely related to the ionic self-diffusion coefficients (see SI Eq. S21), which monotonically decrease with concentration (see SI Figure S12). Consequently, $f_\mathrm{O}$ mirrors the behavior of the self-diffusion coefficients and thus, shows similar decreasing behavior.
Simultaneously, the thermodynamic factor exhibits increasing trends with $c$ and therefore compensates the trends in $f_\mathrm{O}$. This results in relatively balanced diffusion coefficients over the examined concentration range until $D_\pm^\mathrm{VOL}$ is slightly decreasing at $c = 3.0\,\mathrm{M}$ (see SI Figure S5).
The polymer electrolyte shows similar behavior in $f_\mathrm{O}$ and $TDF$, which results in a similar trend for the diffusion coefficient. At elevated concentrations beyond the concentration range used in our MD simulations ($c > 3.0\,\mathrm{M}$), however, the decrease in $f_\mathrm{O}$ becomes more pronounced and dominates the increase in the thermodynamic factor. Thus, the diffusion coefficient monotonically decreases at these concentrations.

## S1.7. Determining the Transport Parameters Using Stefan-Maxwell Diffusivities

In the main text, we relate the electrolyte parameters to combinations of Onsager transport coefficients. Alternatively, these parameters can also be linked to Stefan-Maxwell diffusivities $\mathfrak{D}_{ij}$. Mistry et al. have derived a set of non-linear equations, which connect these diffusivities to relative displacements $\Delta \boldsymbol{r}_{ij}$ of ions and solvent molecules obtained by MD simulations[34]

$$\frac{1}{\Delta}\left(\frac{x_+ + x_-}{\mathfrak{D}_\pm} + \frac{x_- + x_0}{\mathfrak{D}_{-0}} - \frac{x_-}{\mathfrak{D}_{+0}}\right) = \lim_{t\to\infty}\frac{1}{6t}\langle\langle \Delta \boldsymbol{r}_{+0}^2\rangle\rangle \tag{S13}$$

$$\frac{1}{\Delta}\left(\frac{x_+ + x_-}{\mathfrak{D}_\pm} + \frac{x_+ + x_0}{\mathfrak{D}_{+0}} - \frac{x_+}{\mathfrak{D}_{-0}}\right) = \lim_{t\to\infty}\frac{1}{6t}\langle\langle \Delta \boldsymbol{r}_{-0}^2\rangle\rangle \tag{S14}$$

$$\frac{1}{\Delta}\left(\frac{x_+ + x_0}{\mathfrak{D}_{+0}} + \frac{x_- + x_0}{\mathfrak{D}_{-0}} - \frac{x_0}{\mathfrak{D}_\pm}\right) = \lim_{t\to\infty}\frac{1}{6t}\langle\langle \Delta \boldsymbol{r}_{\pm}^2\rangle\rangle \tag{S15}$$

$$\Delta = \frac{x_0}{\mathfrak{D}_{+0}\mathfrak{D}_{-0}} + \frac{x_+}{\mathfrak{D}_{+0}\mathfrak{D}_\pm} + \frac{x_-}{\mathfrak{D}_{-0}\mathfrak{D}_\pm}, \tag{S16}$$

where $x_i$ denotes the mole fraction of species $i$. In this section, we use these equations to calculate the transport parameters of $LiPF_6$ in EC:EMC and compare the results to the transport parameters obtained by the method of Fong et al.[15,33] (see SI Figure S7). As evident in the figure, the parameters obtained by the method of Mistry et al. are quite similar, only the salt diffusion coefficient $D_\pm^\mathrm{COM}$ takes slightly lower values. However, the trends in both parameters sets over temperature and concentration are almost identical.

## S1.8. Radial Distribution Function

In electrolyte systems, solvent molecules surround salt ions, forming solvation shells. The shells induce local fluctuations in the particle densities of the individual solvent species, depending on the distance $r$ to the ion. The radial distribution function (RDF) $g_{i-j}(r)$ compares the time and ensemble averaged density fluctuations $\rho_j(r)$ around an ion species $i$ to the bulk particle density $\rho_j^\mathrm{av} = N_j/V$ of a solvent species $j$, where $N_j$ denotes the corresponding particle number in the electrolyte volume $V$,[35]

$$g_{i-j}(r) = \frac{\rho_j(r)}{\rho_j^\mathrm{av}}. \tag{S17}$$

This provides insights into size and compositions of the solvation shells.
We calculate the RDFs $g_{\mathrm{Li}^+-j}(r)$ and $g_{\mathrm{PF}_6^--j}(r)$ of each electrolyte species $j$ surrounding the $Li^+$ and the $PF_6^-$ ions, respectively. The different ions preferentially interact with different atom groups of the solvent molecules.[36] Therefore, we define $r$ as the distance between the $Li^+$ ion and the carbonyl O atom, and distance between the P atom and the C atoms of the methyl and methylene groups as marked in Figure S8a, respectively. The separation between the $Li^+$ ion and the P atom determines the distance between the ions.

The first minimum after the maxima in the $Li^+$-P RDF typically defines the radius of the inner solvation

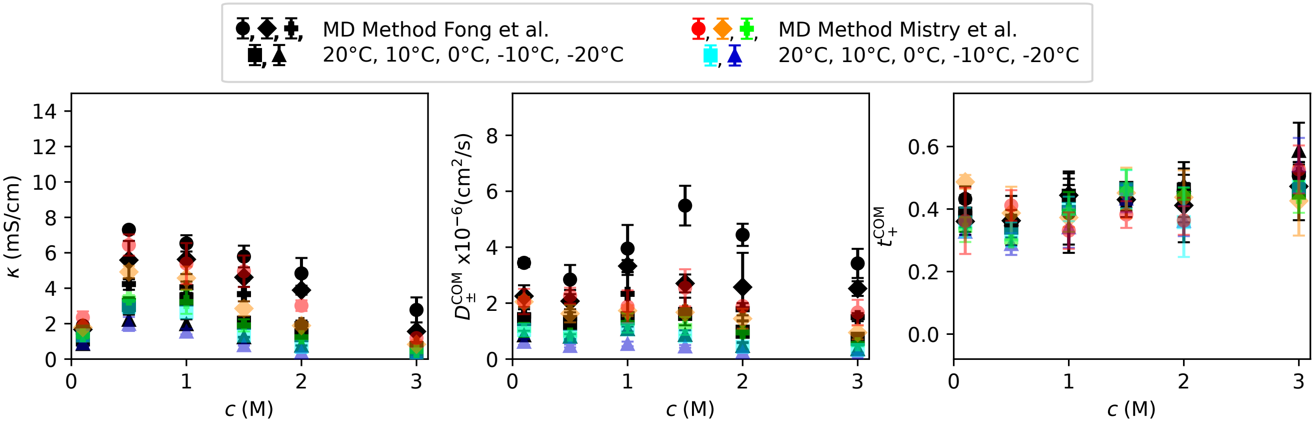


**Figure S7.** Transport parameters of $LiPF_6$ in EC:EMC calculated with the method of Fong et al. and Mistry et al.[15,33,34]

**Table S7.** Averaged radius $r_\mathrm{s}$ of the solvation shell surrounding the $Li^+$ and $PF_6^-$ ions.

| Electrolyte | $r_\mathrm{s}$ (Å) |
|---|---|
| $LiPF_6$ in EC:EMC (3:7, weight) | 5.16 |
| $LiPF_6$ in EC:DMC:PC (27:63:10, volume) | 5.11 |
| $LiPF_6$ in EC:EMC:MP (2:6:2, volume) | 5.16 |

shell $r_\mathrm{s}$ (see SI Figure S8b).[1,15,37,38] Our MD simulations reveal similar radii $r_\mathrm{s}$ for all three examined electrolytes, showing no clear dependence on concentration nor temperature (see SI Figure S9). Therefore, we average the values for each electrolyte, yielding the results listed in Table S7. The averaged radii resemble the findings of Ringsby et al. for 1 M $LiPF_6$ in EC:EMC.[1] Note that the solvation shells of the $Li^+$ and $PF_6^-$ ions are per definition equally sized.
Integrating the RDF $g_{i-j}(r)$ reveals the coordination numbers $n_{i-j}(r_\mathrm{s})$ of the ions in the electrolytes,[35,39]

$$n_{i-j}(r_\mathrm{s}) = 4\pi\rho_j^{\mathrm{av}} \int_0^{r_\mathrm{s}} r^2 g_{i-j}(r)\, dr. \tag{S18}$$

As discussed in Ringsby et al.[1], there are controversial findings regarding the coordination numbers in carbonate based electrolytes, containing EC or PC and acyclic carbonates. While some authors find the $Li^+$ ion solvated preferably or even completely by cyclic molecules,[40–42] others obtain more evenly mixed solvation shells, containing next to EC or PC also linear carbonates.[1,36,43–45] Our MD simulations match with the latter for all our examined electrolytes (see SI Figure S10). Although our EC coordination numbers surpass the number of linear carbonates at low concentrations, they decrease with increasing concentration as similarly described in Ref. 45 for $LiPF_6$ in EC:DMC (1:1, mole ratio). At elevated salt concentrations, the number of EC molecules even undershoots the number of linear carbonates due to a decreasing EC to ion ratio. The linear carbonates show a slight increase in solvation shell population with decreasing

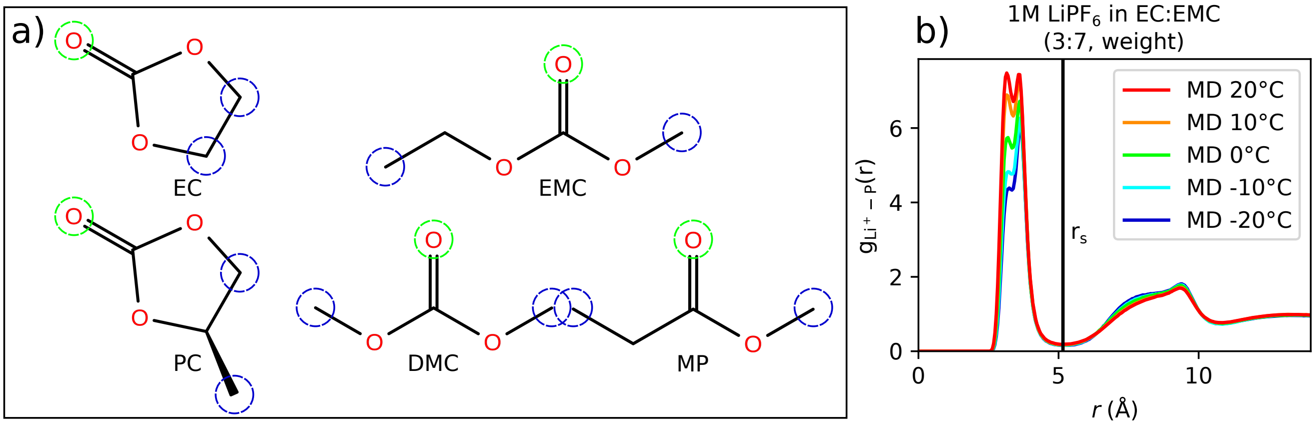


**Figure S8.** a) Structural formulas of the solvent molecules occurring in our electrolytes, generated with Maestro (Schrödinger).[4] The green and blue rings mark the atoms used for calculating the distance $r$ to the $Li^+$ and $PF_6^-$ ions. b) Exemplary RDF function. The solid black line marks the averaged solvation shell radius $r_\mathrm{s}$.

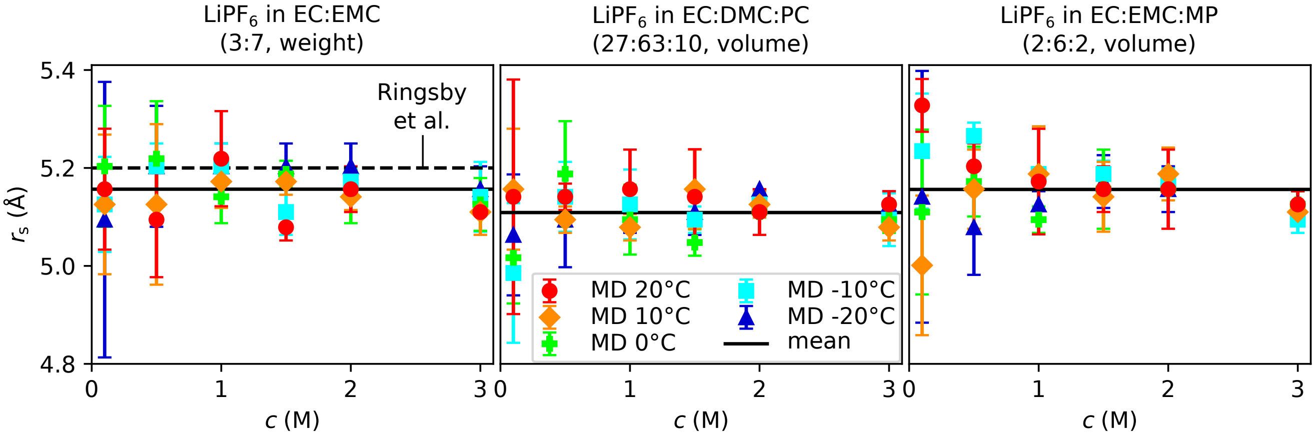


**Figure S9.** Solvation shell radius $r_\mathrm{s}$ of the $Li^+$ and $PF_6^-$ ions, and their corresponding average. Ringsby et al. find similar values for 1 M $LiPF_6$ in EC:EMC.[1]

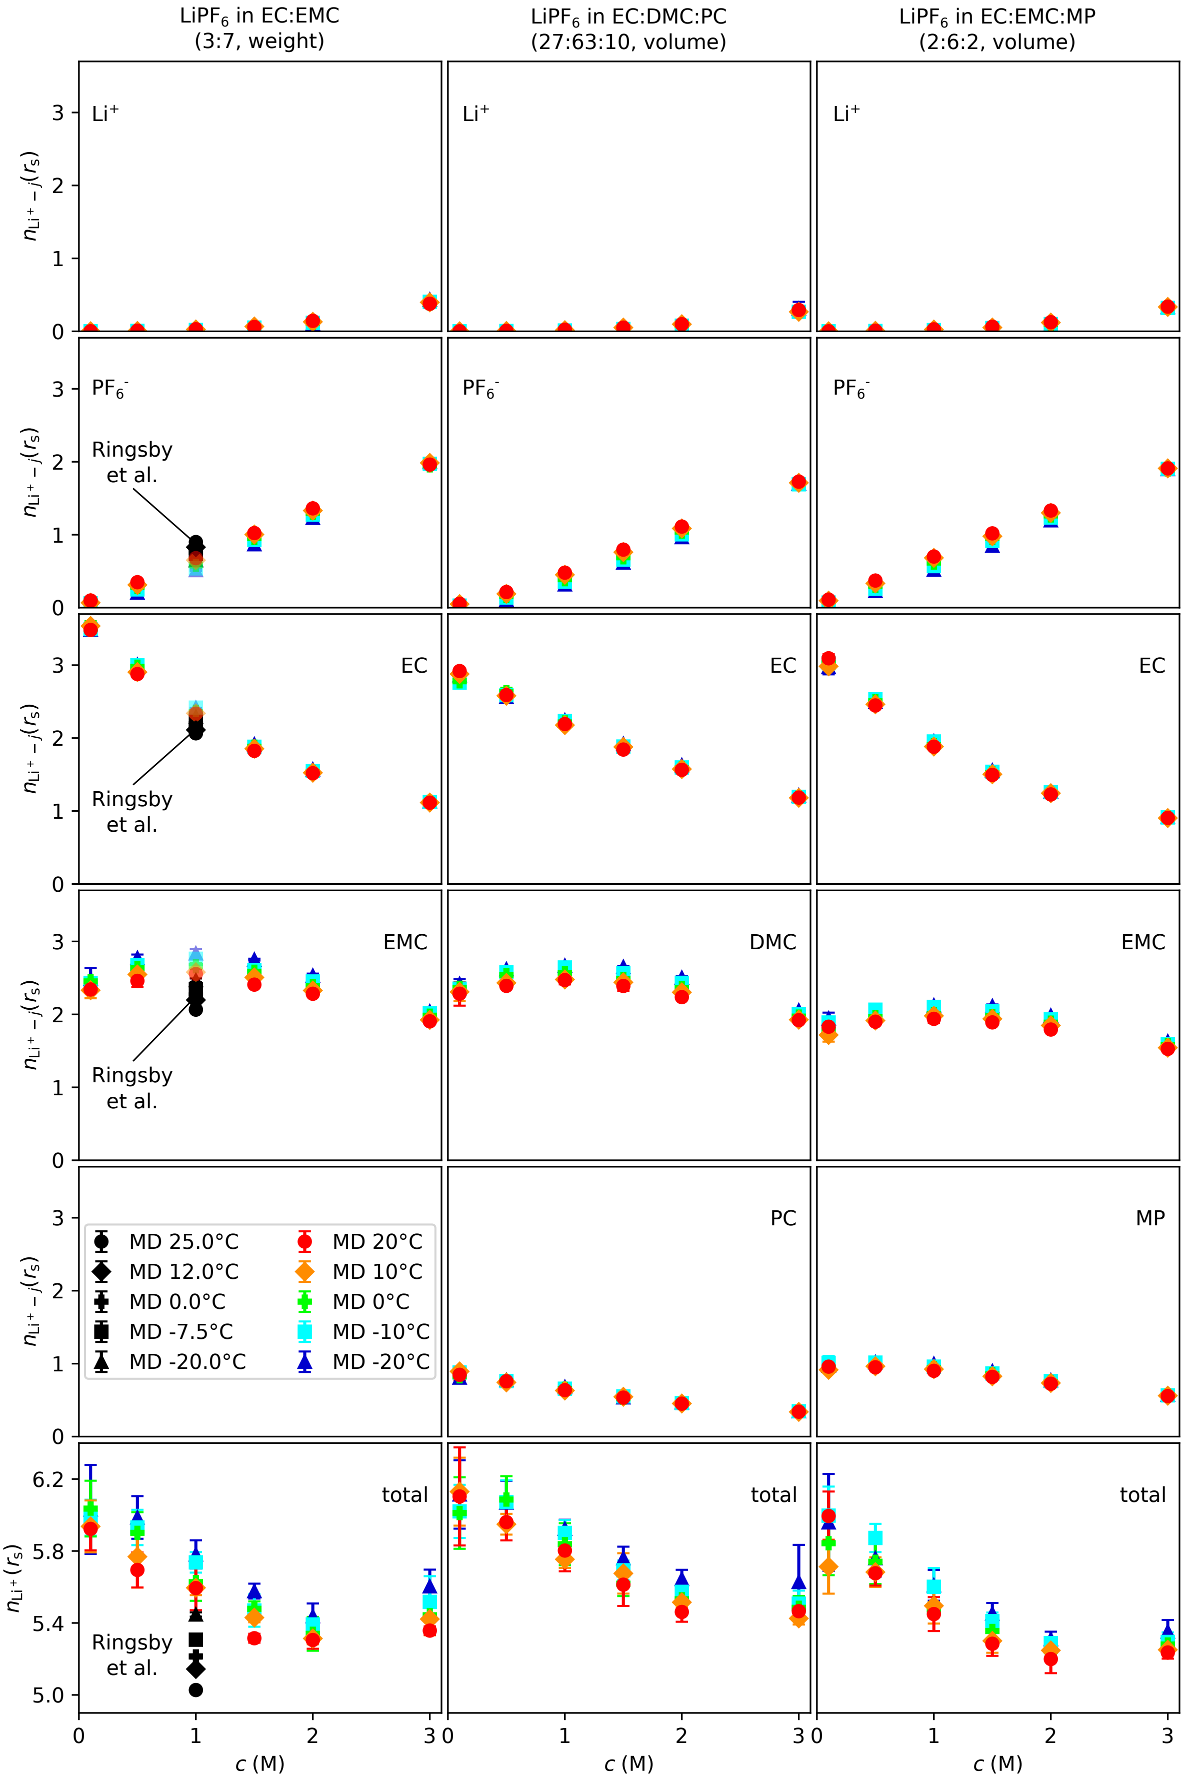


**Figure S10.** Coordination numbers $n_{\mathrm{Li}^+-j}(r_\mathrm{s})$ of the $\mathrm{Li}^+$ ion. The black data points show the MD simulations of Ringsby et al.,[1] using $\zeta = 0.8$.

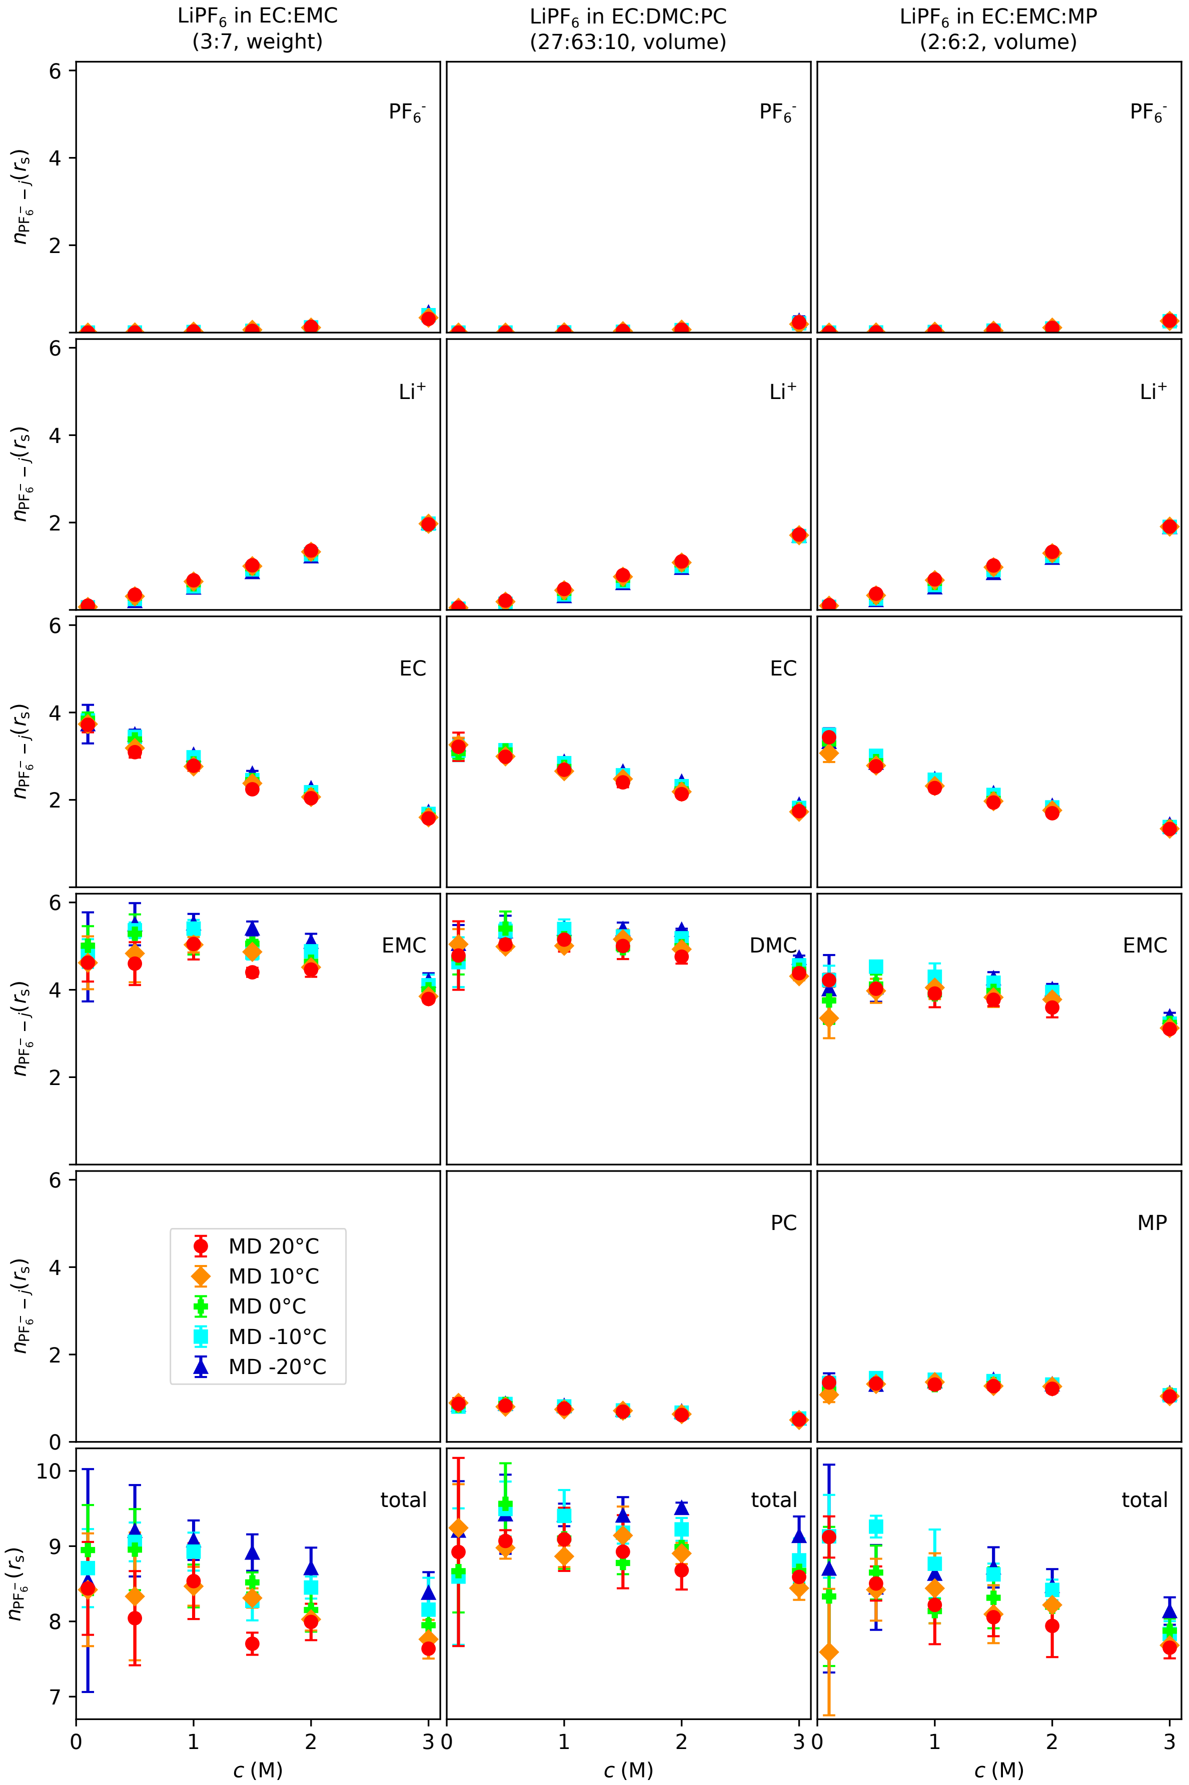


**Figure S11.** Coordination numbers $n_{\mathrm{PF}_6^- - j}(r_\mathrm{s})$ of the $PF_6^-$ ion.

temperature, which could be caused by an increase in solvent permittivity.[1,45] Additionally, the population of $PF_6^-$ increases with concentration and temperature. This is consistent with the results presented in SI Section S1.11.

The coordination numbers of the $PF_6^-$ ion solvation shell show very similar trends, but at higher values and the linear solvents dominating the shell (see SI Figure S11). While the total coordination number for $Li^+$ ranges from 5.2–6.1, it takes values from 7.6–9.6 for $PF_6^-$. This is in accordance with the trends reported in the literature.[1,36,39,44] Note that in the calculation of the coordination number using equation S18, the considered molecules or ions can populate several solvation shells simultaneously, which is especially true at elevated salt concentrations.

## S1.9. Electrolyte Viscosity

The viscosity $\eta$ significantly impacts the ionic transport of electrolytes. Electrolytes with high viscosity are more resistant to deformation, hindering the motion and mobility of the ions.[1] According to the Stokes-Einstein and Nernst-Einstein equation, elevated viscosity values lead to lower conductivities and self-diffusion coefficients, making less viscous electrolytes more desirable.[47,48]

We use the Stokes-Einstein relation to approximate the viscosity for our examined electrolytes in the COM frame. The relation connects the viscosity $\eta$ to the self-diffusion coefficient $D_{\text{self}}^{\text{COM}}$ and the radius $r(c)$ of the electrolyte particles (see Eq. 20). In order to determine $\eta$, we first calculate $D_{\text{self}}^{\text{COM}}$ using our MD simulations and subsequently optimize $r(c)$ using experimental viscosity data.

We define $D_{\text{self}}^{\text{COM}}$ as the composition-weighted average of the individual self-diffusion coefficients $D_{\text{self}}^{i,\text{COM}}$ for each solvent species $i$. To specify $D_{\text{self}}^{i,\text{COM}}$, we consider the Onsager coefficients $L^{ii}$ (see Eq. 3), calculating the cross- ($\alpha \neq \beta$) and autocorrelation function ($\alpha = \beta$) of the particle positions $\boldsymbol{r}_i^{\alpha}(t)$ and $\boldsymbol{r}_i^{\beta}(t)$ with respect to the center-of-mass position. Fong et al. denote these contributions as $L_{\text{distinct}}^{ii}$ and $L_{\text{self}}^{ii}$, capturing the non-ideal interparticle correlation and the ideal Nernst-Einstein transport contributions, respectively,[15]

$$L_{\text{distinct}}^{ii} = \frac{1}{6k_{\text{B}}TV} \lim_{t\to\infty} \frac{\mathrm{d}}{\mathrm{d}t} \left\langle \sum_{\alpha} \left[\boldsymbol{r}_i^{\alpha}(t) - \boldsymbol{r}_i^{\alpha}(0)\right] \cdot \sum_{\beta\neq\alpha} \left[\boldsymbol{r}_j^{\beta}(t) - \boldsymbol{r}_j^{\beta}(0)\right] \right\rangle, \tag{S19}$$

$$L_{\text{self}}^{ii} = \frac{1}{6k_{\text{B}}TV} \lim_{t\to\infty} \frac{\mathrm{d}}{\mathrm{d}t} \left\langle \sum_{\alpha} \left[\boldsymbol{r}_i^{\alpha}(t) - \boldsymbol{r}_i^{\alpha}(0)\right]^2 \right\rangle. \tag{S20}$$

The self-diffusion $D_{\text{self}}^{i,\text{COM}}$ of species $i$ directly relates to the Onsager coefficient contribution $L_{\text{self}}^{ii}$, where $\boldsymbol{r}_i^{\alpha}(t)$ denotes the positions of the corresponding Li, P or carbonyl O atoms with respect to the center-of-mass,

$$D_{\text{self}}^{i,\text{COM}} = \frac{k_{\text{B}}TL_{\text{self}}^{ii}}{c_i}. \tag{S21}$$

The determination of $L_{\text{self}}^{ii}$ follows the same procedure as shown in SI Section S1.3.

Figure S12 shows the self-diffusion coefficients $D_{\text{self}}^{i,\text{COM}}$ of all electrolyte components. For each component, $D_{\text{self}}^{i,\text{COM}}$ increases with temperature but decreases with concentration. The ions show overall lower self-diffusion coefficients compared to the solvents, especially at lower concentrations. This is likely due to the large formation shells, surrounding the ions. Specifically the $Li^+$ ions interact stronger with the solvent molecules (see SI Section S1.11) compared to the $PF_6^-$ ions, leading to lower $D_{\text{self}}^{i,\text{COM}}$. The solvent molecules do mostly not participate in solvation shells and can therefore move more freely, resulting in elevated self-diffusion coefficients at lower concentrations. However, as the concentration increases, a larger fraction of solvent molecules populates the solvation shells. This slows down the solvents, as the bound molecules exhibit slower self-diffusion coefficients compared to the corresponding free bulk molecules,[49] and leads to an overall lower self-diffusion coefficient $D_{\text{self}}^{i,\text{COM}}$ at elevated concentrations. The composition-weighted average of the individual $D_{\text{self}}^{i,\text{COM}}$ reveals $D_{\text{self}}^{\text{COM}}$.

Having identified $D_{\text{self}}^{\text{COM}}$, we now optimize the particle radius $r(c)$ by comparing the calculated viscosities to experimental data (see SI Figure S13). Experimental viscosity measurements have already been conducted for $LiPF_6$ in EC:EMC.[46] However, to the knowledge of the authors, there are no measurements available for $LiPF_6$ in EC:DMC:PC and in EC:EMC:MP.

Ringsby et al.[1] have found, that the solvent particle radius for the electrolytes 1 M $LiPF_6$ in EC:EMC (3:7, weight), in GBL:EMC (3:7, weight) and in EC:GBL:EMC (15:15:70, weight) varies less than 2%. Therefore, we approximatively use the same $r(c)$ optimized for $LiPF_6$ in EC:EMC for all our three electrolytes. Note that this introduces additional un-

**Table S8.** Fit parameter $\eta_0$ and the activation energy $E_{\text{a}}$ of $\eta_{\text{exp}}$ for $LiPF_6$ in EC:EMC.

| $c$ (m) | $\eta_0$ (cP) | $E_{\text{a}}$ (J/mol) |
|---|---|---|
| 0.5 | $9.175\cdot10^{-3}$ | $1.300\cdot10^{4}$ |
| 1.0 | $4.414\cdot10^{-3}$ | $1.613\cdot10^{4}$ |
| 1.5 | $1.256\cdot10^{-3}$ | $2.079\cdot10^{4}$ |
| 2.0 | $6.016\cdot10^{-4}$ | $2.404\cdot10^{4}$ |

**Table S9.** Fit parameters $m_{\text{r}}$ and $r_0$ of the particle radius $r(c)$ for $LiPF_6$ in EC:EMC.

| $m_{\text{r}}$ (Å/M) | $r_0$ (Å) |
|---|---|
| −0.65 | 2.78 |

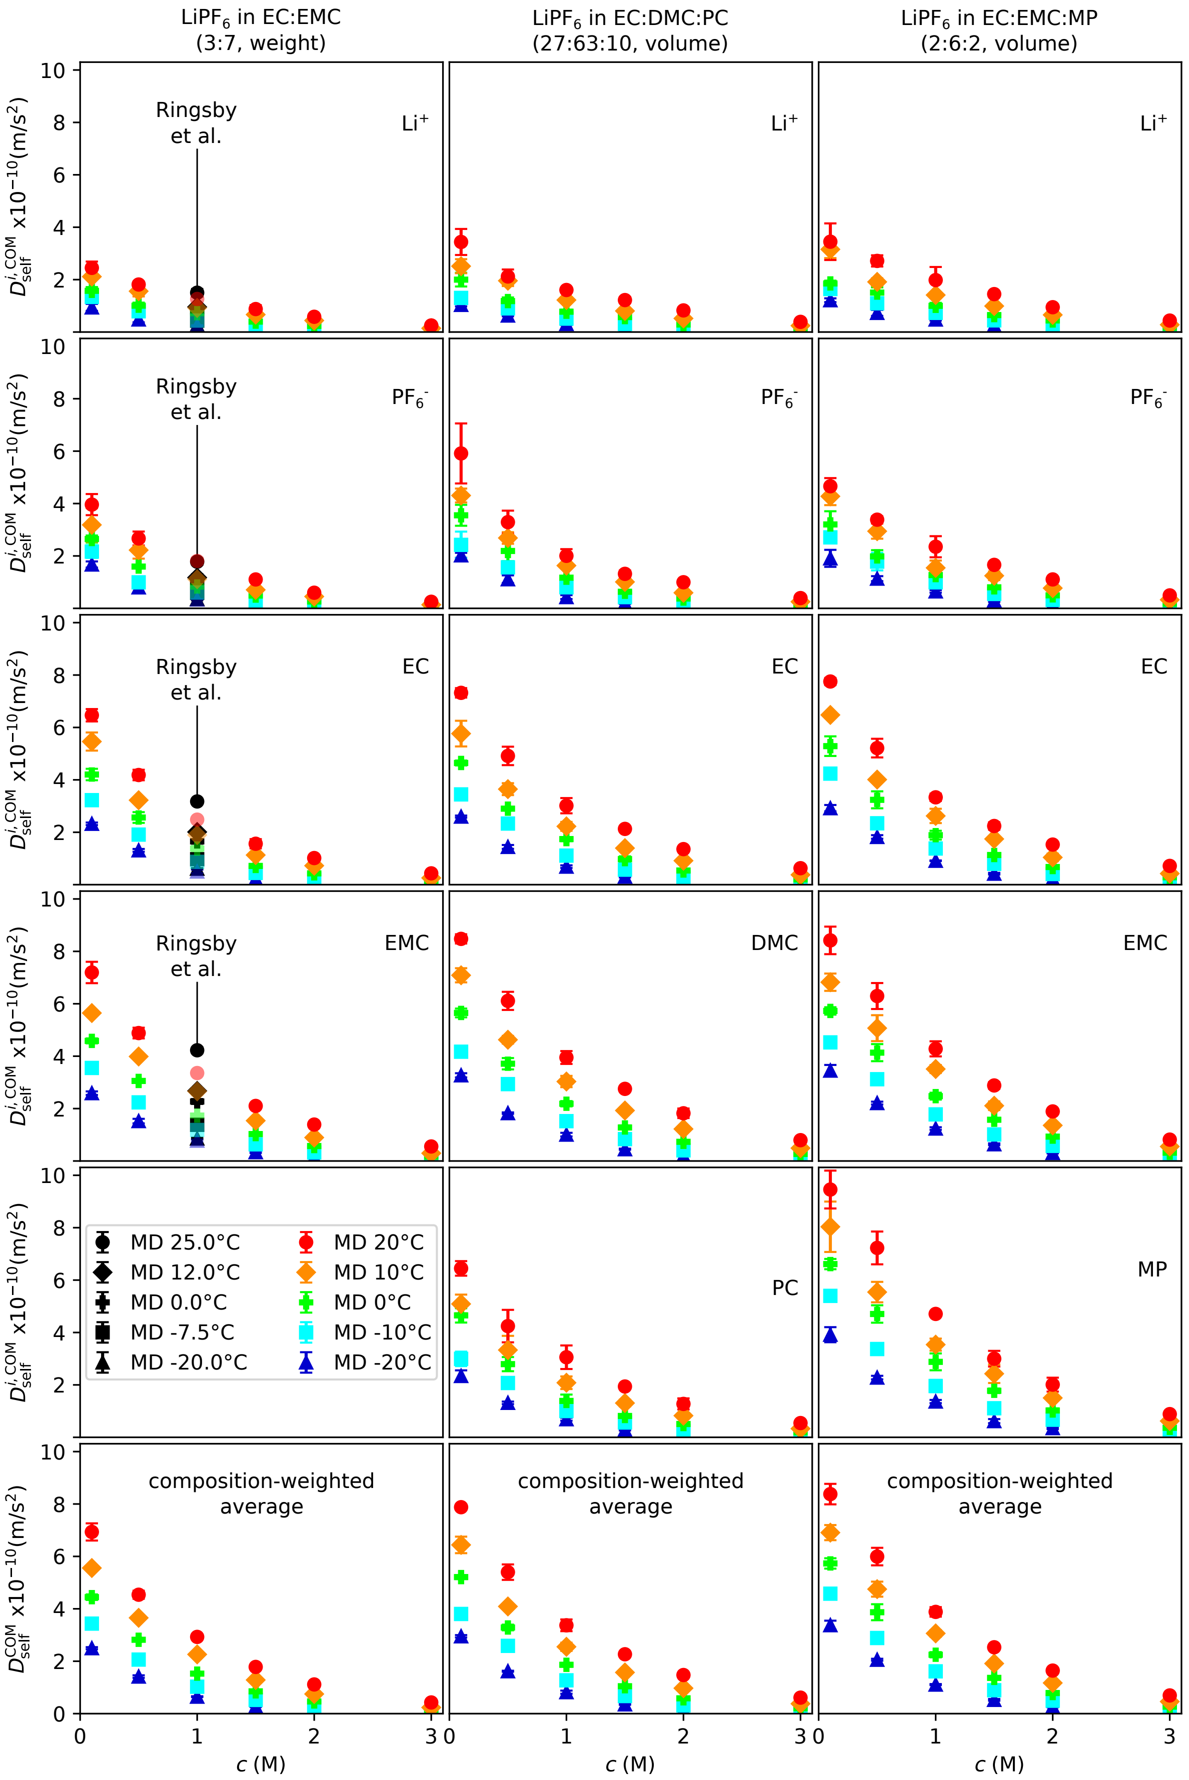


**Figure S12.** Self-diffusion coefficients $D_{\mathrm{self}}^{i,\mathrm{COM}}$ for the respective species $i$, and the corresponding composition-weighted average $D_{\mathrm{self}}^{\mathrm{COM}}$. The black data points show the MD simulation results of Ringsby et al.,[1] using $\zeta = 0.8$.

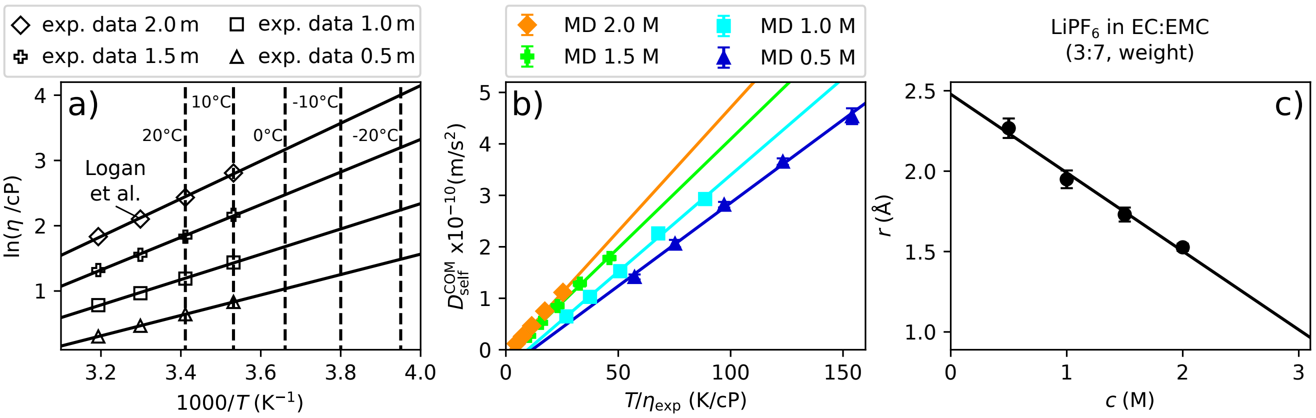


**Figure S13.** a) Viscosity data of Logan et al.[46] and the corresponding Arrhenius fits $\eta_{\text{exp}}$ for $LiPF_6$ in EC:EMC. b) Composition-weighted averaged self-diffusion coefficient $D_{\text{self}}^{\text{COM}}$ over $T/\eta_{\text{exp}}$ with their corresponding fits. The slope $m$ reveals the particle radius $r(c)$. c) Particle radius $r(c)$ and its corresponding linear fit.

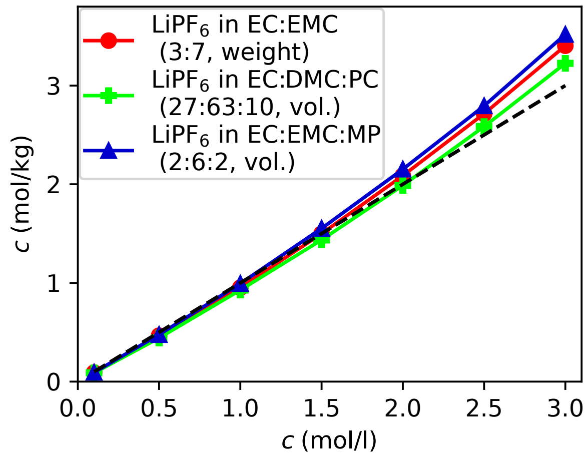


**Figure S14.** Molal concentration over molar concentration. Both measures are similar, especially for $c \leq 2.0\,\text{M}$. The dashed line indicates identical behavior.

certainty to the imprecise viscosity approximations of the Stokes-Einstein relation for multicomponent electrolytes.

Logan et al. provides experimental viscosity data for $LiPF_6$ in EC:EMC at $c \leq 2.0\,\text{m}$ and $T \geq 10\,°\text{C}$.[46] Fitting the data to an Arrhenius equation[50] (see Eq. S22) by using the fit parameter $\eta_0$ and the activation energy $E_{\text{a}}$ allows for extrapolating the viscosity to lower temperatures (see SI Figure S13a and SI Table S8),

$$\eta_{\text{exp}} = \eta_0 \exp \frac{E_{\text{a}}}{RT}. \tag{S22}$$

For the optimization of $r(c)$, we plot $D_{\text{self}}^{\text{COM}}$ over $T/\eta_{\text{exp}}$ and linearly fit the data with a function of the form $f(x) = mx + b$ (see SI Figure S13b). The slope $m$ reveals $r(c)$ with

$$r(c) = \frac{k_{\text{B}}}{6\pi m}. \tag{S23}$$

Linearly fitting the obtained particle radii with $r(c) = m_{\text{r}}c + r_0$ enables estimating $r(c)$ at higher and lower concentrations (see SI Figure S13c and SI Table S9). Note that the concentration in the viscosity experiments in Ref. 46 is measured in molal (m) in contrast to our calculations, being in molar (M). However, the conversion of mol/kg in mol/l yields for the considered electrolytes similar values, especially for $c \leq 2.0\,\text{M}$ (see SI Figure S14).

Finally, the insertion of $D_{\text{self}}^{\text{COM}}$ and $r(c)$ into the Stokes-Einstein relation determines the viscosity shown in Figure 5. Note that Ringsby et al. calculate the solvent viscosity, using the composition-weighted average of the self-diffusion coefficients of the solvent species to isolate viscosity effects on the electrolyte transport from the influence of ion association.[1] For our electrolytes, however, the electrolyte viscosity hardly deviates from the solvent viscosity (see SI Figure S15).

## S1.10. Residence Time and Diffusion Length

The residence time $\tau_i$ defines for how long a solvent molecule of species $i$ stays within the first solvation shell of an ion. The duration depends on the diffusion mechanism and the solvent viscosity.[1,51]

In order to determine $\tau_i$, we calculate the distances between the ions and atoms as described in SI Section S1.8 for each time frame of the MD simulation. If the distance between the ion $k$ and the solvent molecule $l$ is smaller than the first solvation shell radius $r_{\text{s}}$, the corresponding adjacency matrix $H_i^{kl}(t') = 1$. Otherwise, we set $H_i^{kl}(t') = 0$. Averaging the autocorrelation functions of the individual adjacency matrices over each ion of species $j$ and each solvent molecule of species $i$ yields the lifetime correlation function $P_i^j(t)$,[52]

$$P_i^j(t) = \left\langle \frac{1}{N_{\text{ion}} N_i} \sum_k^{N_{\text{ion}}} \sum_l^{N_i} H_i^{kl}(t') H_i^{kl}(0) \right\rangle. \tag{S24}$$

The point in time, when $P_i^j(t) \leq 0.1$ defines the residence time $\tau_i$. In some simulations, the residence time takes longer durations than our production runs. For

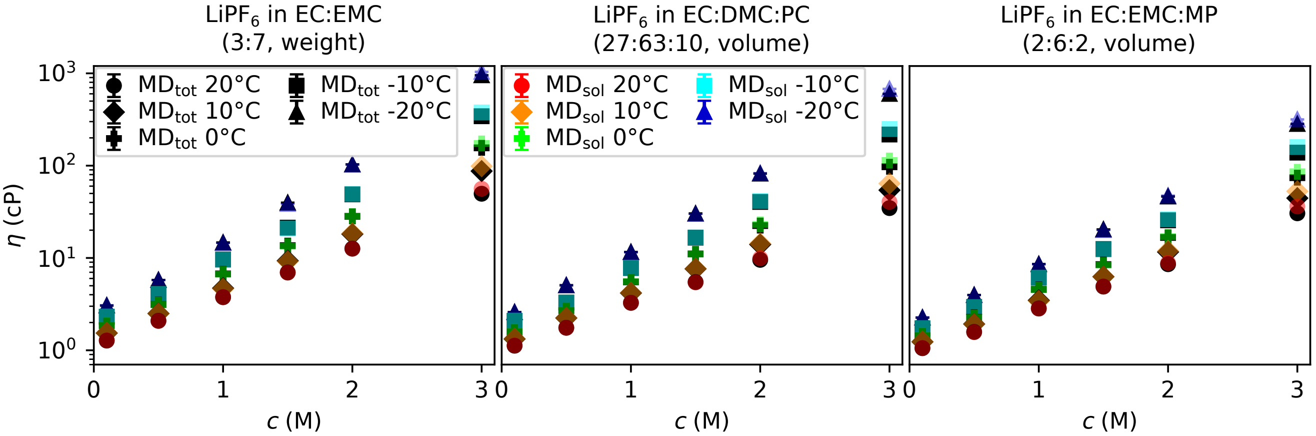


**Figure S15.** Calculated electrolyte viscosity (black data points) and solvent viscosity (colored data points), using MD simulations. Both viscosities are almost identical.

these simulations, we extrapolate the residence time by fitting an exponential function to the autocorrelation data at long times $t$, where $\ln P_i^j(t) \propto t$. This avoids fitting data points corresponding to faster, sub-diffusive processes (see SI Figure S16).[51]

Figures S17 and S18 show the residence times $\tau_i$ for our three electrolytes. $\tau_i$ resembles the trends of the viscosity $\eta$, as it increases with concentration and decreasing temperature for all solvent species. While the cyclic solvents EC and PC reside for the longest times in the ion solvation shell of both $Li^+$ and $PF_6^-$, the $PF_6^-$ shell shows overall shorter $\tau_i$.

Calculating the diffusion length $L_i$ isolates the influence of the diffusion process on the residence time[1,38,51]

$$L_i = \sqrt{6 D_{\mathrm{self,sol}}^{\mathrm{COM}} \tau_i}, \tag{S25}$$

where $D_{\mathrm{self,sol}}^{\mathrm{COM}}$ denotes the composition-averaged self-diffusion coefficient of the solvent molecules. $L_i$ measures the distance, for which the solvent molecules of species $i$ escort the considered ion before it leaves

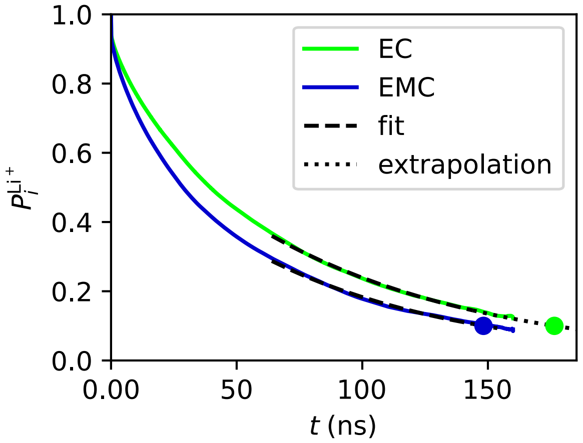


**Figure S16.** Exemplary evaluation of the lifetime correlation function $P_i^{\mathrm{Li}^+}(t)$ for 3 M $LiPF_6$ in EC:EMC at $T = -20\,°\mathrm{C}$. In order to calculate $\tau_i$, we extrapolate $P_i^{\mathrm{Li}^+}(t)$ using an exponential function.

the corresponding solvation shell. While long diffusion lengths hint towards vehicular type diffusion with stable solvation shells, short $L_i$ indicate faster, structural type diffusion, where the ions rapidly exchange their solvation shell molecules.[1,38,51,53,54]

Figures S19 and S20 show the diffusion lengths of the solvent species in the $Li^+$ and $PF_6^-$ ion solvation shells. The cyclic carbonates EC and PC exhibit elevated values in $L_i$ with decreasing trends with temperature and concentration. In contrast, the linear carbonates DMC, EMC and MP, reveal shorter diffusion lengths and less pronounced trends, especially for the solvents surrounding the $PF_6^-$ ion. This suggests stronger interactions between the cyclic carbonates and the ions,[49] which could be attributed to their elevated dipole moments compared to the linear carbonates.[55–58] The decreasing trend with concentration could be explained by an increasing ion to solvent molecule ratio, where more and more ions compete for the same number of solvent molecules.[59] This could lead to a more rapid exchange of the solvent molecules between solvation shells rather than a slower exchange between solvation shell and the bulk electrolyte. $L_i$ takes overall lower values for the solvent molecules in the solvation shell of the $PF_6^-$ ion compared to the $Li^+$ ion. Therefore, the solvent molecules exhibit weaker interactions with the $PF_6^-$ ion, which could be due to a lower charge density of the $PF_6^-$ ion and of the positive dipole end of the solvent molecule.[44,59]

In order to estimate the changes in the diffusion type over concentration and temperature, we calculate the composition-weighted average of $L_i$ for both ions (see Figure 6).

## S1.11. Ion Association

In concentrated electrolytes, the ion solvation shell can comprise next to solvent molecules also other ions, leading to the formation of ion associations. This can severely impact the ionic transport of the electrolytes. We analyze the formation of ion associations for our

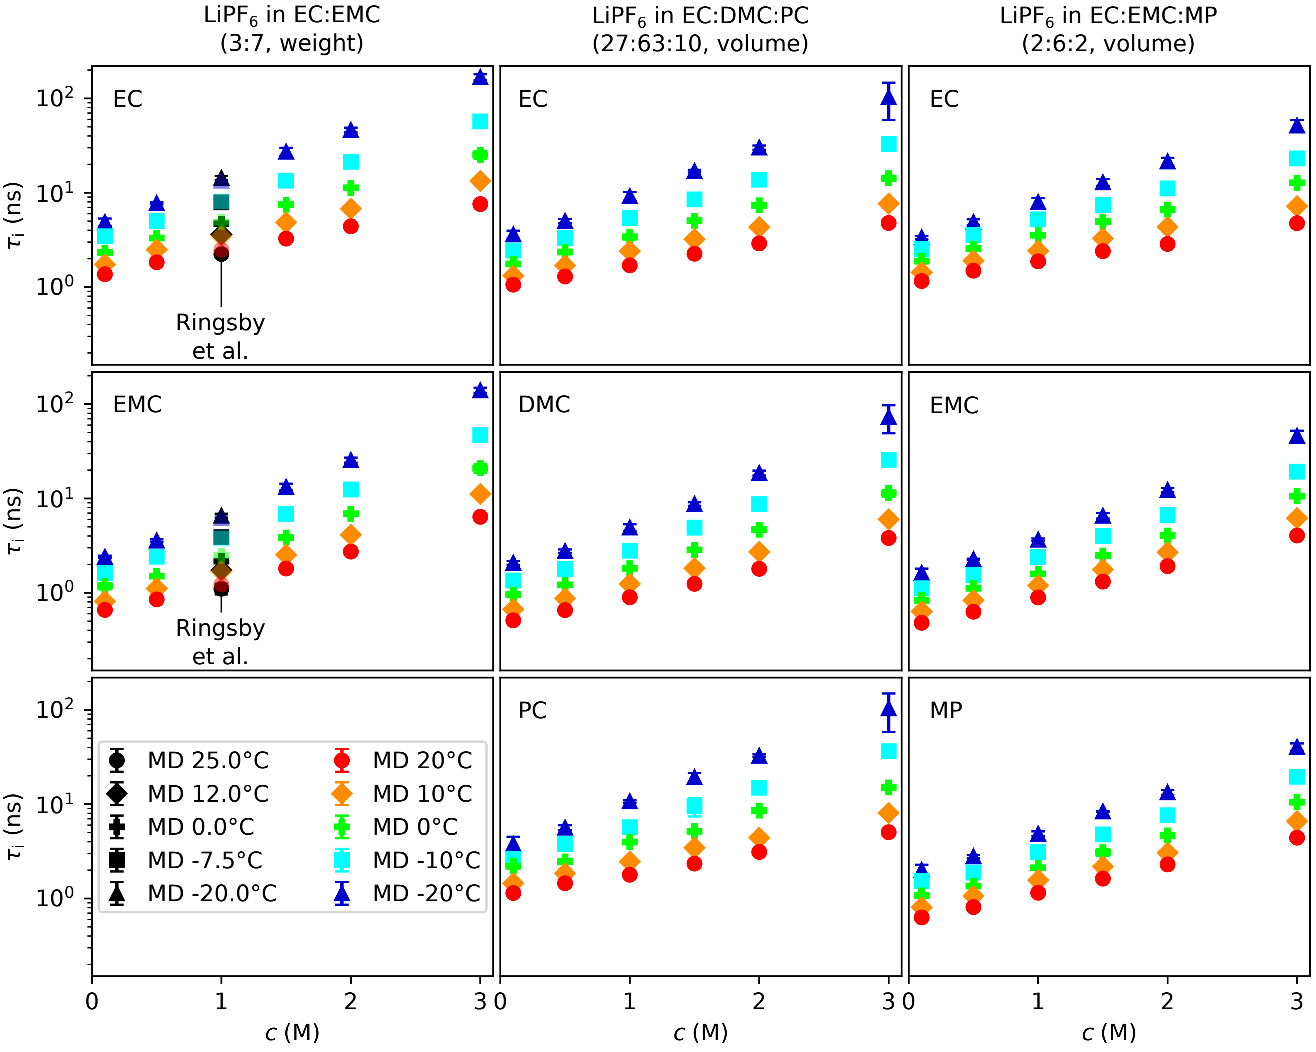


**Figure S17.** Residence time $\tau_i$ of the solvent molecules of species $i$, populating the $Li^+$ solvation shell. The data matches the MD calculations of Ringsby et al. for 1 M $LiPF_6$ in EC:EMC, using $\zeta = 0.8$.[1]

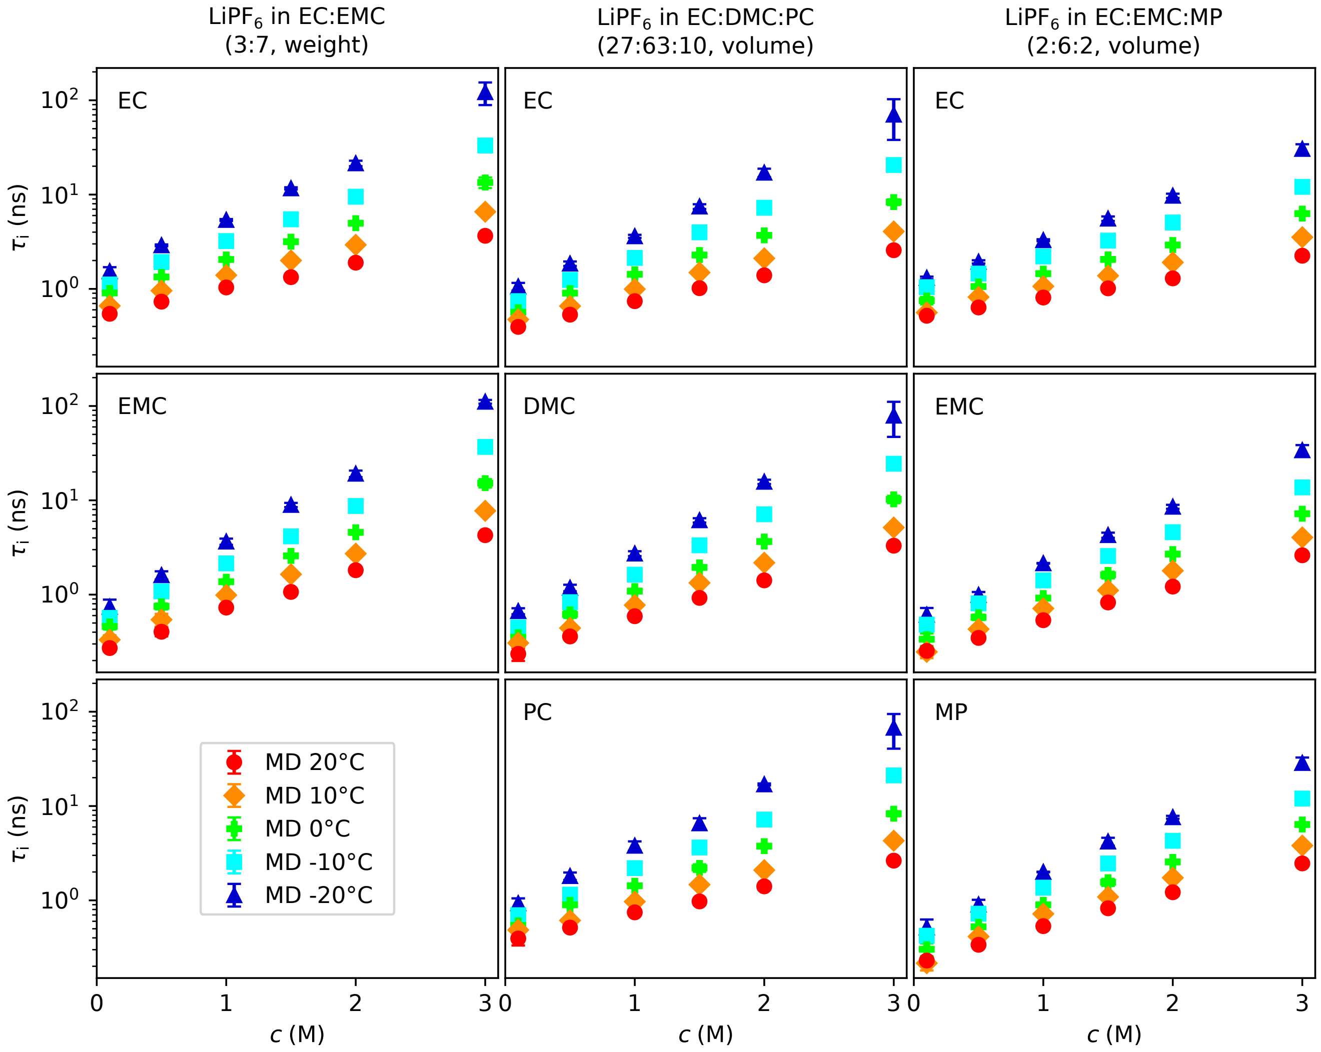


**Figure S18.** Residence time $\tau_i$ of the solvent molecules of species $i$, populating the $PF_6^-$ solvation shell.

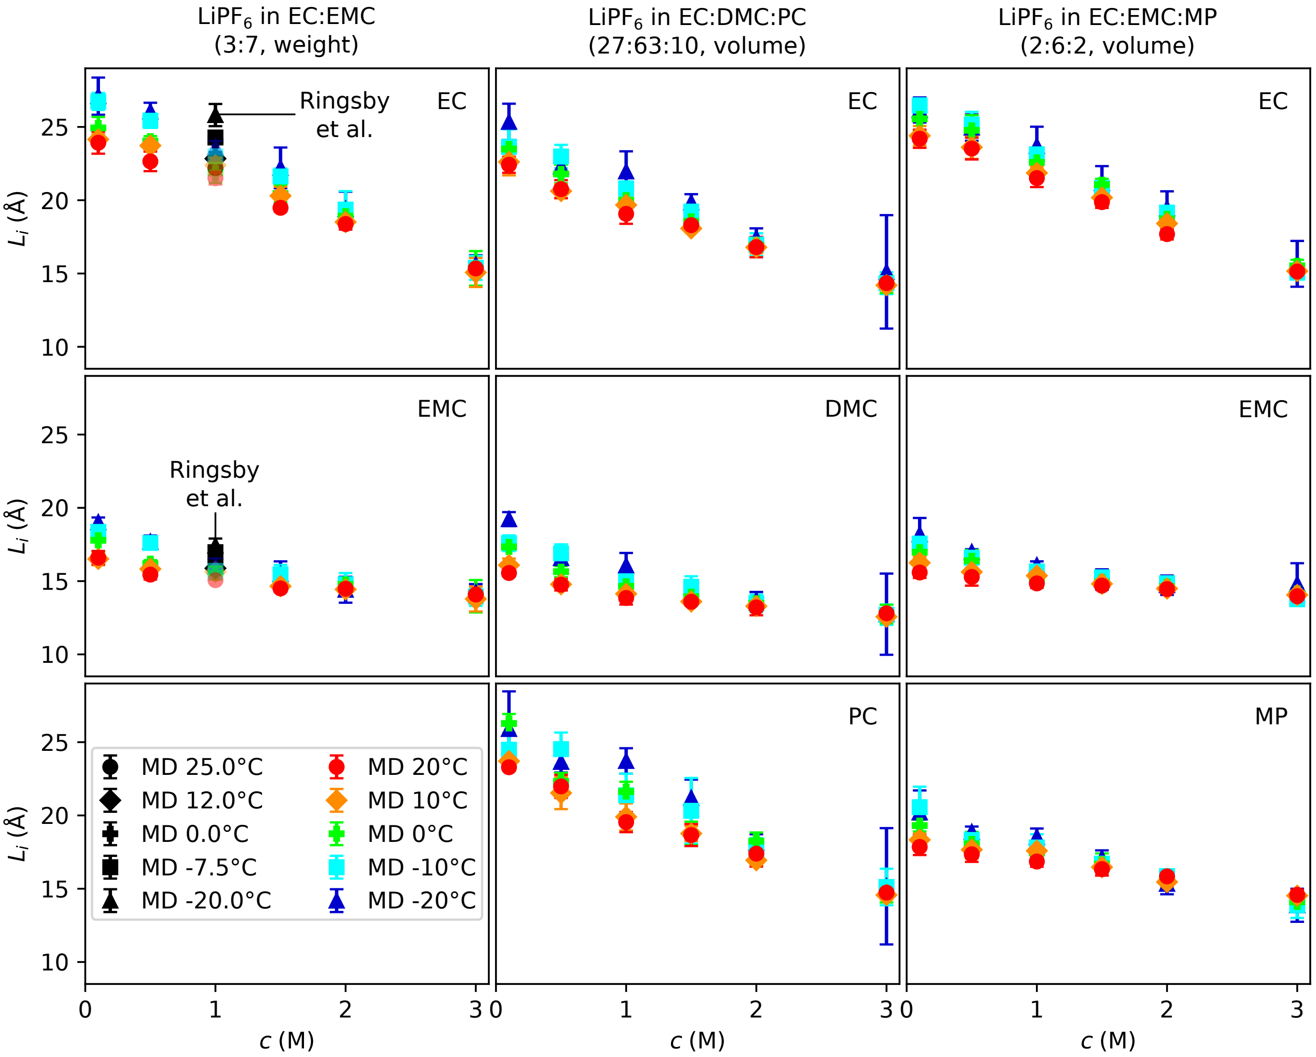


**Figure S19.** Diffusion length $L_i$ of the solvent molecules of species $i$, populating the $Li^+$ solvation shell. The data matches the MD calculations of Ringsby et al. for 1 M $LiPF_6$ in EC:EMC, using $\zeta = 0.8$.[1]

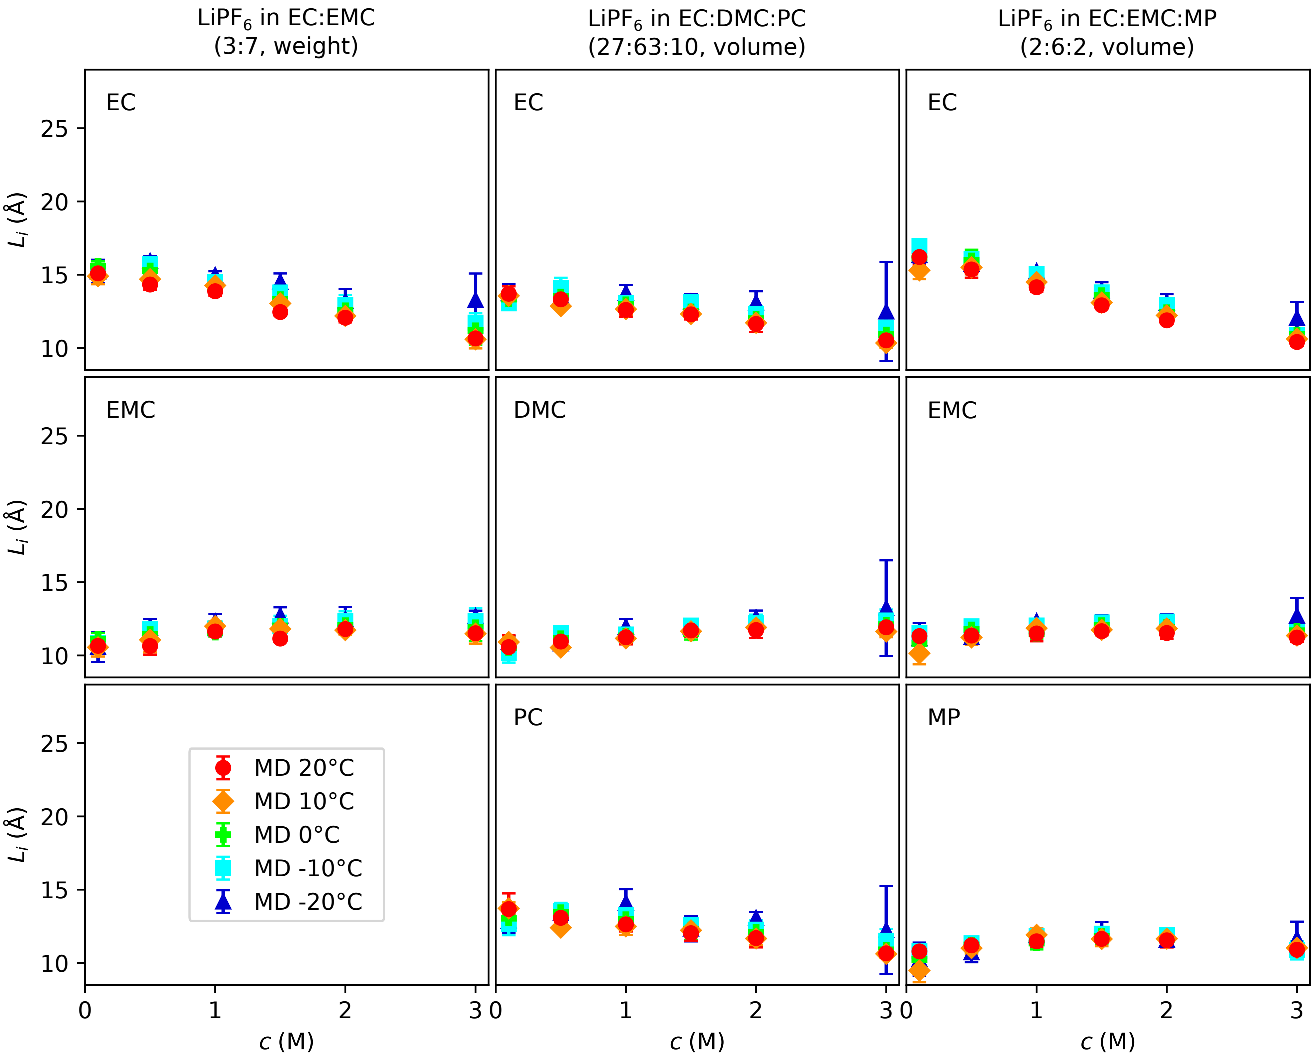


**Figure S20.** Diffusion length $L_i$ of the solvent molecules of species $i$, populating the $PF_6^-$ solvation shell.

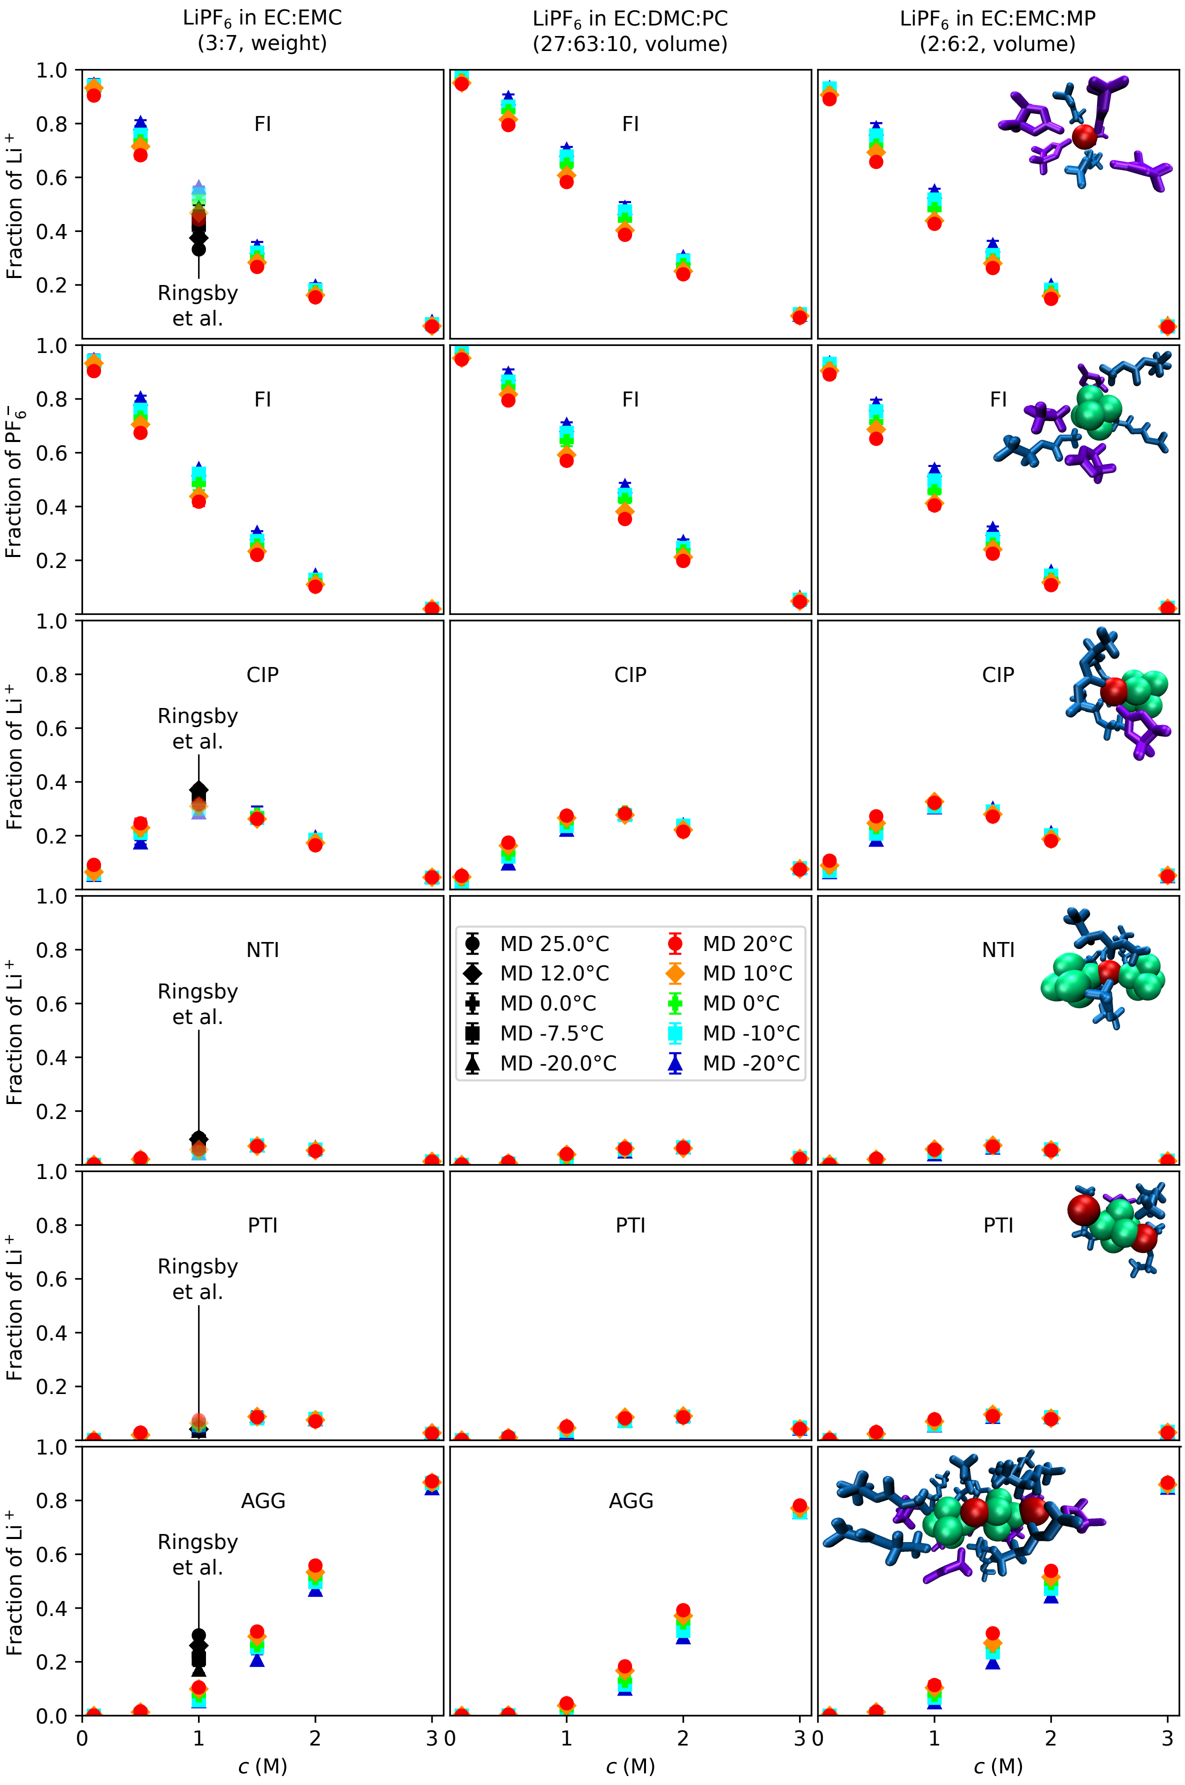


**Figure S21.** Fraction of $Li^{+}$ and $PF_6^{-}$ ions in the different ion associations. The black data points show the MD simulations of Ringsby et al.,[1] using $\zeta = 0.8$.

three electrolytes, using our MD simulations. For this, we calculate the distances between all $Li^+$ and $PF_6^-$ ions. An ion is part of an association, if its distance to another ion or member of an ionic cluster is smaller than the the inner solvation shell radius $r_s$ (see SI Section S1.8).
$Li^+$ and $PF_6^-$ ions without any other ions in their solvation shell are considered as free (FI). Depending on the cluster composition, the associations further classify into contact ion pairs (CIP: $Li^+ + PF_6^-$), negative and positive triple ions (NTI: $Li^+ + 2\,PF_6^-$ and PTI: $2\,Li^+ + PF_6^-$) and larger aggregates (AGG).[1]
Calculating the respective time averaged number of $Li^+$ or $PF_6^-$ ions in each category yields the results shown in SI Figure S21. The formation of aggregates increases with temperature and concentration. This leads to a maximum in the concentration of free ions at low temperatures and intermediate salt concentrations (see Figure 7). Although the total number of NTIs is slightly higher than the number of PTIs, only a negligibly small number of triple ions is formed for all three of our electrolytes.
The temperature dependence can be explained by multiple contrary contributions.[1,60] Lowering the temperature enlarges the Bjerrum length, describing the maximum distance at which the electrostatic energy of the ions exceeds the thermal energy.[61] Therefore, the formation of ion associations should be enhanced. In contrast, the dipole alignment of the solvent molecules is less thermally perturbed. This leads to elevated dielectric permittivities and more stable solvent solvation shells, impeding the formation of ion associations.[60] Additionally, Ringsby et al. discuss an entropic effect:[1] Although the formation of ion associations reduces the entropy of the ions, it simultaneously increases the entropy of the released solvent molecules, detaching from the solvation shell into the bulk electrolyte. This can lead to an overall entropic gain, which is more prominent at low temperatures.[62]
The dependence on increasing salt concentration can be explained by a larger ion to solvent molecule ratio, improving the formation probability of ion associations.

## S1.12. Electrophoretic Mobility

The electrophoretic mobility $u = \frac{v}{E}$ relates the ion-specific migration drift velocity $v$ to the applied electric field $E$. Determining the electrophoretic mobilities $u_+$ and $u_-$ for the $Li^+$ and $PF_6^-$ ions allows for calculating the transference number (see Eq. 16).
We calculate the mobilities $u_+$ and $u_-$ in the COM frame, using MD simulations and compare the results to the transformed findings of the eNMR measurements (see SI Figure S22). Note that for the transformation of the experimental findings, we employed the same coefficients $\Psi_i$ (see SI Table S4) as used for the transformation of the simulation results in Eq. S7. The simulations match the experimental results fairly well, both exhibiting a decreasing trend with concentration and decreasing temperature.
Analyzing the obtained trends allows for estimating the dependencies of the mobility. The mobility depends on

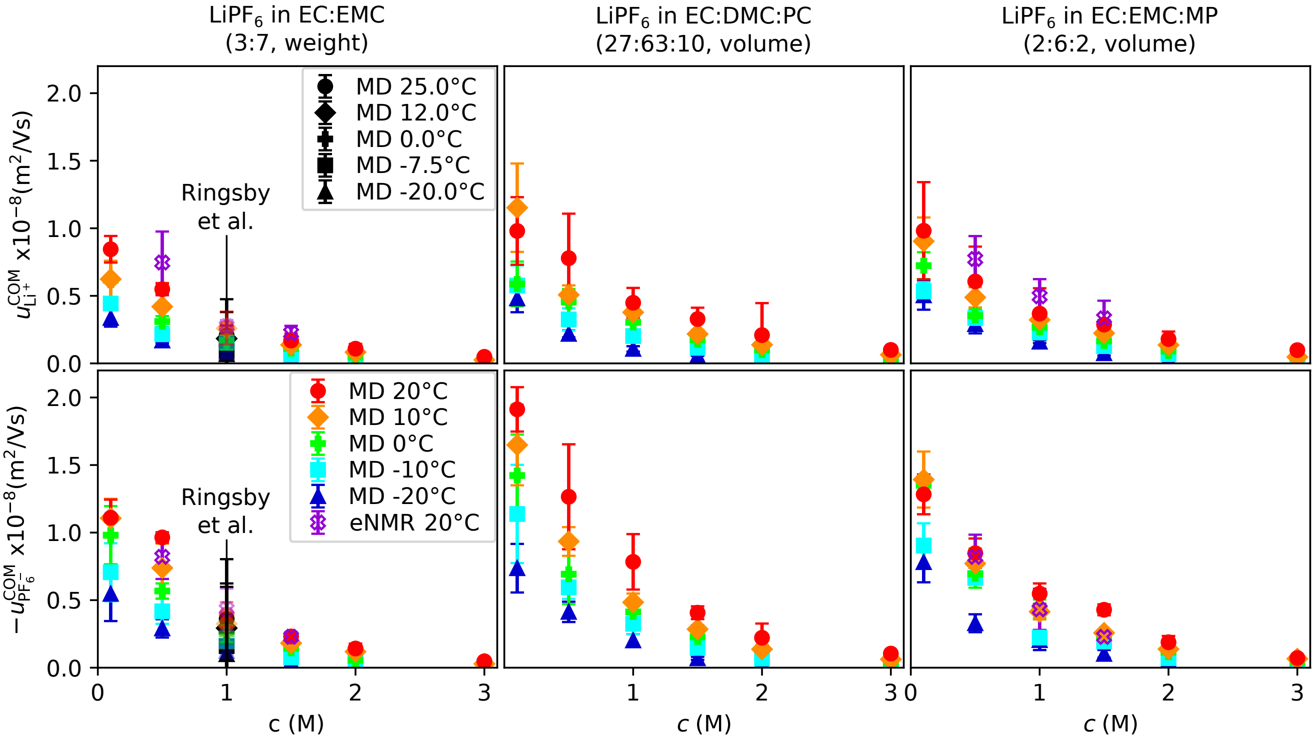


**Figure S22.** Electrophoretic mobilities $u$ of the $Li^+$ and the $PF_6^-$ ions for our three electrolytes in the COM frame. The black data points show the MD simulations of Ringsby et al.,[1] using $\zeta = 0.8$.

the viscosity $\eta$ and the prevalent diffusion mechanism of the ions. While both viscosity and diffusion mechanism indicate increasing mobilities with temperature for all three electrolytes, they imply opposite trends with concentration (see Figures 5 and 6). The decreasing mobility with concentration is in line with the expectations based on the viscosity. This suggests that for our electrolytes, the viscosity has a greater impact on the electrophoretic mobilities than the diffusion mechanism.

# S2. Experiments

## S2.1. Experimental Details

In order to precisely determine the four parameters for our electrolytes, we combine our MD simulations with two kinds of electrochemical experiments: EIS measuring the conductivity $\kappa$ and concentration cells specifying $a^{\mathrm{VOL}}(c,T)$ (see Eqs. 12, 13). Additionally, eNMR measurements are conducted for the electrolytes $LiPF_6$ in EC:EMC and in EC:EMC:MP to benchmark the calculated transference numbers $t_+$.

For preparing the experiments, we purchased $LiPF_6$ (Solvionic, 99.99% battery grade), EC (Alfa Aesar, anhydrous, 99%), EMC (Solvionic, battery grade), MP (Alfa Aesar, 99%) and metallic Li-foil (Alfa Aesar, 750 µm thickness, 99.9%). All required electrolyte mixing tools and cell parts for the electrochemical experiments underwent an overnight heating protocol prior to the electrolyte preparation and the subsequent cell assembly in argon-filled glove boxes (Jacomex GPT4FF, <1 ppm $H_2O$, <3 ppm $O_2$ and GS Glovebox Systemtechnik GmbH MEGA E-Line, <1 ppm $H_2O$, <1 ppm $O_2$). The EIS and concentration cell measurements were performed in a climate chamber (Vötsch Industrietechnik GmbH, LabEvent L T/64/40/3), using Zennium Pro and Zahner IM6 potentiostats (Zahner-Elektrik GmbH). Additional details can be found in Ref. 63.

*Conductivity Cell*

As mentioned above, optimizing our MD simulations requires benchmarking the simulated conductivities with experimental data. The comparison allows for adjusting the scaling factor $\zeta$ (see SI Table S3) and thus, for more accurate simulation results.

In order to measure the conductivity of $LiPF_6$ in EC:EMC:MP, we conducted EIS measurements using the airtight TSC 1600 closed cell and the software RelaxIS (both from rhd instruments). Further experimental details can be found in previous work.[63] Conductivity values for $LiPF_6$ in EC:EMC and in EC:DMC:PC are already available in the literature.[22,25]

*Concentration Cell*

Concentration cells measure convoluted information about the transference number and the thermodynamic factor in form of $a^{\mathrm{VOL}}(c,T)$ (see Eqs. 11–13). Therefore, combining MD simulations with concentration cell measurements enables a complete determination of the four electrolyte parameters (see Eqs. 4–6, 14).

In order to measure $a^{\mathrm{VOL}}(c,T)$ for $LiPF_6$ in EC:EMC:MP, we use custom concentration cells. We measure the potential difference $U_{\mathrm{c}}$ between two Li metal electrodes immersed in electrolytes with slightly deviating concentrations $c = c_0 \pm \delta c$ at various temperatures $T$. In our experiments, we use $\delta c = 0.19\,\mathrm{M}$ for the lowest and $\delta c = 0.25\,\mathrm{M}$ for all remaining base concentrations $c_0$. Fitting the obtained potentials with equation 13 yields the coefficients $a_i(T)$ and thus, reveals $a^{\mathrm{VOL}}(c,T)$ (see Eq. 12). Further details on the experimental set-up are described in previous work.[63] Concentration cell data for the electrolytes $LiPF_6$ in EC:EMC and in EC:DMC:PC are found in the literature.[22,25]

*eNMR*

Electrophoretic NMR experiments were conducted on an AVANCE Neo 400 MHz NMR spectrometer with a respective DiffBB gradient probe head (Bruker, Ettlingen, Germany). The probe head provides a maximum magnetic gradient strength of 17 T/m. The temperature was set to 20 °C. The eNMR sample cell with electrodes is a custom design described previously.[64] A double-stimulated echo sequence is applied[65] to avoid convective artefacts, employing fixed values of $\Delta \leq 50\,\mathrm{ms}$, $\delta = 1\,\mathrm{ms}$ and $g \leq 240\,\mathrm{G/cm}$, depending on the sample. The pulse sequence contains two voltage pulses with alternating sign, applied by a power source from P&L Scientific (Lidingö, Sweden). In subsequent spectra the voltage is incremented linearly up to a maximum value of $U \leq 80\,\mathrm{V}$. The resulting phase shift is linearly fitted in dependence on voltage as described earlier.[64] For each nucleus ($^7$Li, $^{19}$F) and sample at least three independent experiments were performed and the resulting electrophoretic mobilities were averaged. Corresponding errors are the sum of fitting errors, statistical errors and an additional error contribution of 5 %.

## S2.2. Concentration Cell Measurements

The full determination of the four electrolyte parameters requires next to the MD simulations experimental results of concentration cells. Measuring the concentration potential $U_{\mathrm{c}}$ allows for the determination of $a^{\mathrm{VOL}}(c,T)$, comprising convoluted information about the transference number $t_+$ and the thermodynamic factor *TDF* (see Eqs. 11–14). While Landesfeind et al. and Valøen et al. provide the desired potentials for $LiPF_6$ in EC:EMC and in EC:DMC:PC,[22,25] we conduct concentration cell measurements for $LiPF_6$ in EC:EMC:MP.

Figure S23 shows the averaged potential difference $U_{\mathrm{c}}$ of two identical cells for various concentrations and temperatures. As evident in the Figure, lower and higher concentrations are missing data points at cooler temperatures. At these concentration-temperature pairs, the potential $U_{\mathrm{c}}$ measured between the half-cells ex-

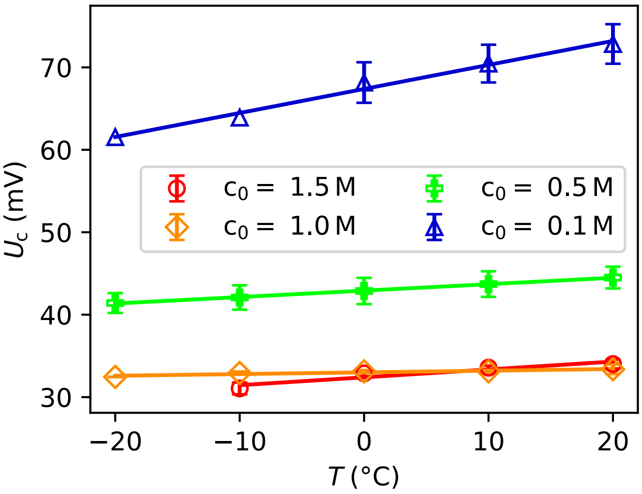


**Figure S23.** Measured potential difference $U_c$ of $LiPF_6$ in EC:EMC:MP using concentration cells with various base concentrations $c_0$ at different temperatures. The errorbars represent the standard deviation of two identical cells. Data without errorbars comprise only one usable concentration cell measurement. The solid lines serve as guidelines for the eyes.

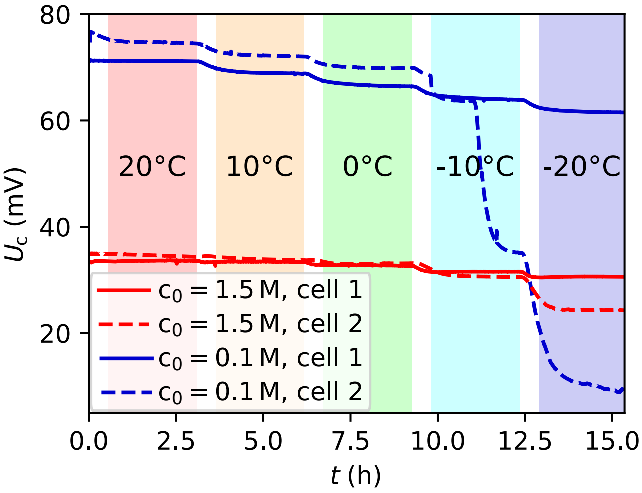


**Figure S24.** Measured potential $U_c$ for each two identical concentration cells with base concentrations $c_0 = 0.1\,M$ and $c_0 = 1.5\,M$. At temperatures below $T \leq -10\,°C$, $U_c$ shows deviating values for the identical cells.

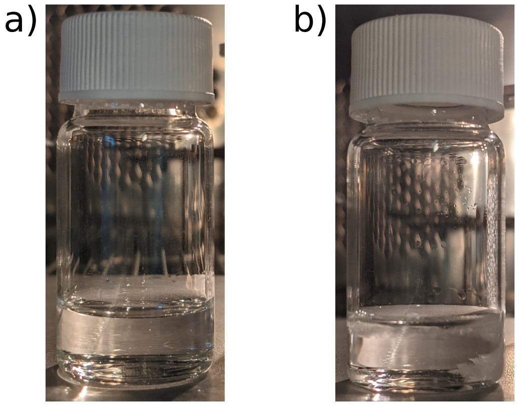


**Figure S25.** 0.1 M $LiPF_6$ in EC:EMC:MP at $-30\,°C$ before a) and after b) being shaken, inducing ice formation.

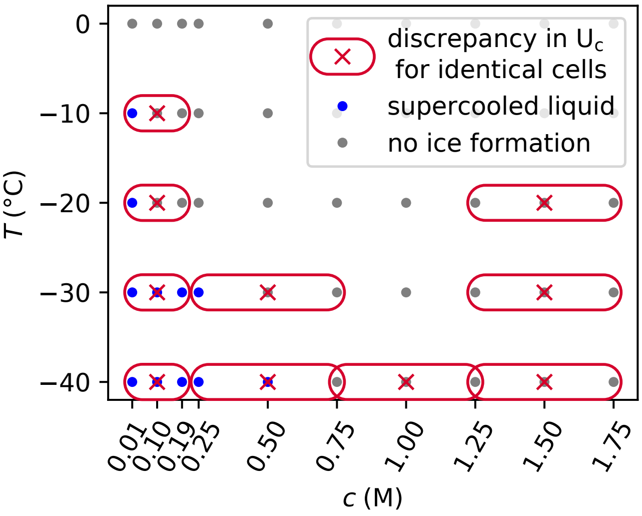


**Figure S26.** Testing the electrolyte for supercooled liquids at varying concentrations and temperatures. The red crosses mark the base concentrations $c_0$ for which the corresponding concentration cells show different potentials $U_c$ for identical cells. The boxes indicate the used concentrations in the half-cells.

hibits significantly deviating values for identical concentration cells (see Figure SI S24).

For low concentrations, this phenomenon can be explained by supercooling. In some but not all identical half-cells, the electrolyte nucleates and forms solid ice crystals, probably consisting of solid EC due to its relatively high melting point. This changes the effective concentrations in the corresponding half-cells, altering $U_c$ depending on the amount of the formed ice. Therefore, we only evaluate the data of the purely liquid concentration cells.

To roughly test at which temperatures the used concentrations enter the supercooled state, we stepwise cool down the corresponding test-blends. After tempering the electrolytes for several hours at each temperature step, we shake the glass vessels to activate nucleation. Any formed ice indicates, that the electrolyte was supercooled (see SI Figure S25). Figure S26 summarizes the results.

For elevated concentrations at lower temperatures, $U_c$ deviates for identical concentration cells as well. However, no ice crystals form within these blends. Therefore, the authors suspect that the salt solubility decreases with decreasing temperature. Salting-out could modify the electrolyte concentrations in the half-cells and affect $U_c$.

## S2.3. Representative eNMR Phaseshifts

The eNMR measurements capture the phase shift $\phi - \phi_0$ over the applied voltage $U$ (see Eq. 15). Linearly fitting the data allows for determining the slope, revealing the electrophoretic mobility $u^{VOL}$ using equation 15. This allows for determining the transference numbers of the ions (see Eq. 16).

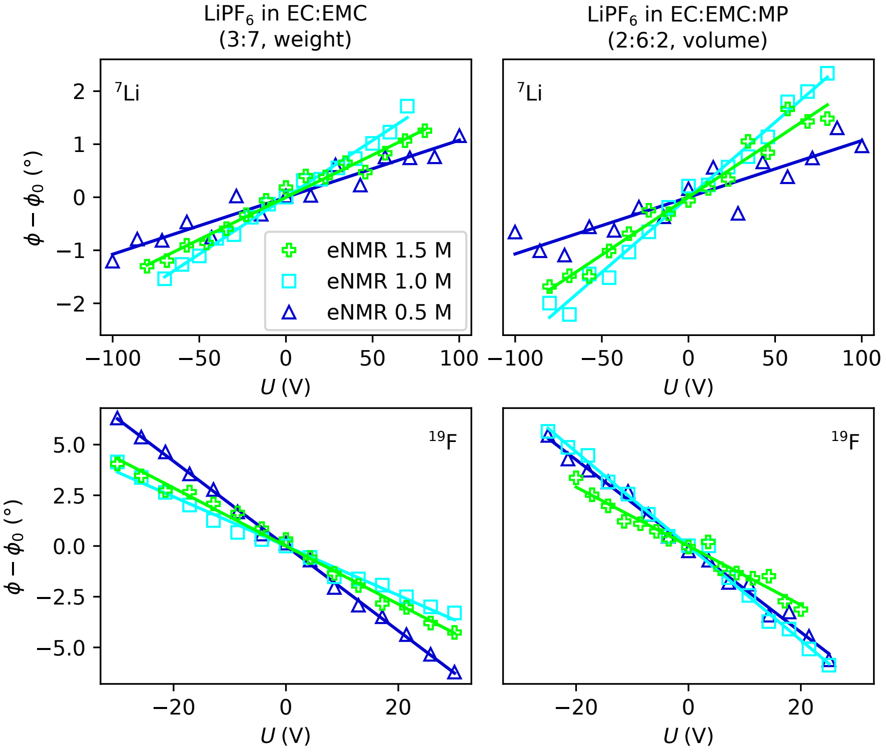


**Figure S27.** Phase shift $\phi - \phi_0$ over the applied voltage $U$ at 20 °C. The slope of the corresponding linear fits reveals the electrophoretic mobility $u$ of the considered atoms in the VOL frame.

Figure S27 shows representative eNMR data together with the corresponding linear fits for our electrolytes at $0.5\,\mathrm{M} \leq c \leq 1.5\,\mathrm{M}$ and $T = 20\,^{\circ}\mathrm{C}$.

## References


[1] A. J. Ringsby, K. D. Fong, J. Self, H. K. Bergstrom, B. D. McCloskey, K. A. Persson, *Journal of The Electrochemical Society* **2021**, *168*, 080501.

[2] A. P. Thompson, H. M. Aktulga, R. Berger, D. S. Bolintineanu, W. M. Brown, P. S. Crozier, P. J. in 't Veld, A. Kohlmeyer, S. G. Moore, T. D. Nguyen, R. Shan, M. J. Stevens, J. Tranchida, C. Trott, S. J. Plimpton, *Computer Physics Communications* **2022**, *271*, 108171.

[3] J. L. Banks, H. S. Beard, Y. Cao, A. E. Cho, W. Damm, R. Farid, A. K. Felts, T. A. Halgren, D. T. Mainz, J. R. Maple, R. Murphy, D. M. Philipp, M. P. Repasky, L. Y. Zhang, B. J. Berne, R. A. Friesner, E. Gallicchio, R. M. Levy, *Journal of Computational Chemistry* **2005**, *26*, 1752.

[4] *Schrödinger Release 2021-1:Maestro, Schrödinger, LLC, New York, NY* **2021**.

[5] K. P. Jensen, W. L. Jorgensen, *Journal of Chemical Theory and Computation* **2006**, *2*, 1499.

[6] J. N. Canongia Lopes, A. A. H. Pádua, *The Journal of Physical Chemistry B* **2004**, *108*, 16893.

[7] V. Chaban, *Physical Chemistry Chemical Physics* **2011**, *13*, 16055.

[8] L. Martínez, R. Andrade, E. G. Birgin, J. M. Martínez, *Journal of Computational Chemistry* **2009**, *30*, 2157.

[9] S. Nosé, *Molecular Physics* **1984**, *52*, 255.

[10] S. Nosé, *The Journal of Chemical Physics* **1984**, *81*, 511.

[11] W. G. Hoover, *Physical Review A* **1985**, *31*, 1695.

[12] W. G. Hoover, *Physical Review A* **1986**, *34*, 2499.

[13] W. C. Swope, H. C. Andersen, P. H. Berens, K. R. Wilson, *The Journal of Chemical Physics* **1982**, *76*, 637.

[14] R. W. Hockney, *Computer simulation using particles*, A. Hilger **1989**.

[15] K. D. Fong, J. Self, B. D. McCloskey, K. A. Persson, *Macromolecules* **2020**, *53*, 9503.

[16] K. D. Fong, *https://github.com/kdfong/transport-coefficients-MSD*.

[17] N. Michaud-Agrawal, E. J. Denning, T. B. Woolf, O. Beckstein, *Journal of Computational Chemistry* **2011**, *32*, 2319.

[18] R. J. Gowers, M. Linke, J. Barnoud, T. J. Reddy, M. N. Melo, S. L. Seyler, J. Domanski, D. L. Dotson, S. Buchoux, I. M. Kenney, et al., MDAnalysis: a Python package for the rapid analysis of molecular dynamics simulations, in *Proceedings of the 15th python in science conference* **2016** page 105.

[19] Sigma-Aldrich®, *https://www.sigmaaldrich.com*.

[20] M. H. Kowsari, S. Alavi, B. Najafi, K. Gholizadeh, E. Dehghanpisheh, F. Ranjbar, *Physical Chemistry Chemical Physics* **2011**, *13*, 8826.

[21] A. Savitzky, M. J. E. Golay, *Analytical Chemistry*

**1964**, *36*, 1627.
[22] L. O. Valøen, J. N. Reimers, *Journal of The Electrochemical Society* **2005**, *152*, A882.
[23] D. S. Hall, J. Self, J. R. Dahn, *The Journal of Physical Chemistry C* **2015**, *119*, 22322.
[24] R. Naejus, D. Lemordant, R. Coudert, P. Willmann, *The Journal of Chemical Thermodynamics* **1997**, *29*, 1503.
[25] J. Landesfeind, H. A. Gasteiger, *Journal of The Electrochemical Society* **2019**, *166*, A3079.
[26] A. Latz, J. Zausch, *Journal of Power Sources* **2011**, *196*, 3296.
[27] A. Latz, J. Zausch, *Beilstein Journal of Nanotechnology* **2015**, *6*, 987.
[28] M. Schammer, B. Horstmann, A. Latz, *Journal of The Electrochemical Society* **2021**, *168*, 026511.
[29] M. Schammer, *Transport theory for highly correlated electrolytes with non-local species interactions*, Ph.D. thesis **2023**.
[30] H. Lundgren, M. Behm, G. Lindbergh, *Journal of The Electrochemical Society* **2014**, *162*, A413.
[31] C. L. Berhaut, P. Porion, L. Timperman, G. Schmidt, D. Lemordant, M. Anouti, *Electrochimica Acta* **2015**, *180*, 778.
[32] K. W. Gao, N. P. Balsara, *Solid State Ionics* **2021**, *364*, 115609.
[33] K. D. Fong, H. K. Bergstrom, B. D. McCloskey, K. K. Mandadapu, *AIChE Journal* **2020**, *66*.
[34] A. Mistry, Z. Yu, L. Cheng, V. Srinivasan, *Journal of The Electrochemical Society* **2023**, *170*, 110536.
[35] J.-P. Hansen, I. R. McDonald, *Theory of Simple Liquids*, Elsevier Science & Technology Books **1990**.
[36] M. H. C. Peiris, S. Brennan, D. Liepinya, H. Liu, M. Smeu, *Colloids and Surfaces A: Physicochemical and Engineering Aspects* **2023**, *674*, 131831.
[37] C. Fang, D. M. Halat, A. Mistry, J. A. Reimer, N. P. Balsara, R. Wang, *Chemical Science* **2023**, *14*, 5332.
[38] J. Self, K. D. Fong, K. A. Persson, *ACS Energy Letters* **2019**, *4*, 2843.
[39] S. Han, *Scientific Reports* **2017**, *7*.
[40] A. von Cresce, K. Xu, *Electrochemical and Solid-State Letters* **2011**, *14*, A154.
[41] K. Xu, A. von Wald Cresce, *Journal of Materials Research* **2012**, *27*, 2327.
[42] K. Xu, Y. Lam, S. S. Zhang, T. R. Jow, T. B. Curtis, *The Journal of Physical Chemistry C* **2007**, *111*, 7411.
[43] D. M. Seo, S. Reininger, M. Kutcher, K. Redmond, W. B. Euler, B. L. Lucht, *The Journal of Physical Chemistry C* **2015**, *119*, 14038.
[44] M. T. Ong, O. Verners, E. W. Draeger, A. C. T. van Duin, V. Lordi, J. E. Pask, *The Journal of Physical Chemistry B* **2015**, *119*, 1535.
[45] O. Borodin, M. Olguin, P. Ganesh, P. R. C. Kent, J. L. Allen, W. A. Henderson, *Physical Chemistry Chemical Physics* **2016**, *18*, 164.
[46] E. R. Logan, E. M. Tonita, K. L. Gering, J. R. Dahn, *Journal of The Electrochemical Society* **2018**, *165*, A3350.
[47] K. L. Gering, *Electrochimica Acta* **2006**, *51*, 3125.
[48] N. Yao, L. Yu, Z. Fu, X. Shen, T. Hou, X. Liu, Y. Gao, R. Zhang, C. Zhao, X. Chen, Q. Zhang, *Angewandte Chemie International Edition* **2023**, *62*.
[49] L. Yang, A. Xiao, B. L. Lucht, *Journal of Molecular Liquids* **2010**, *154*, 131.
[50] C. Berhaut, D. Lemordant, P. Porion, L. Timperman, G. Schmidt, M. Anouti, *RSC Advances* **2019**, *9*, 4599.
[51] K. D. Fong, J. Self, K. M. Diederichsen, B. M. Wood, B. D. McCloskey, K. A. Persson, *ACS Central Science* **2019**, *5*, 1250.
[52] C. J. F. Solano, S. Jeremias, E. Paillard, D. Beljonne, R. Lazzaroni, *The Journal of Chemical Physics* **2013**, *139*.
[53] T. P. Liyana-Arachchi, J. B. Haskins, C. M. Burke, K. M. Diederichsen, B. D. McCloskey, J. W. Lawson, *The Journal of Physical Chemistry B* **2018**, *122*, 8548.
[54] M. Forsyth, H. Yoon, F. Chen, H. Zhu, D. R. MacFarlane, M. Armand, P. C. Howlett, *The Journal of Physical Chemistry C* **2016**, *120*, 4276.
[55] D. Orbakh, *Nonaqueous electrochemistry*, Marcel Dekker **1999**.
[56] R. Nagl, Z. Fan, C. Nobis, C. Kiefer, A. Fischer, T. Zhang, T. Zeiner, M. Fischlschweiger, *Journal of Molecular Liquids* **2023**, *386*, 122449.
[57] B. P. Kar, N. Ramanathan, K. Sundararajan, K. Viswanathan, *Journal of Molecular Structure* **2014**, *1072*, 61.
[58] H. Lee, S. Hwang, M. Kim, K. Kwak, J. Lee, Y.-K. Han, H. Lee, *The Journal of Physical Chemistry Letters* **2020**, *11*, 10382.
[59] K. L. Gering, *Electrochimica Acta* **2017**, *225*, 175.
[60] M. S. Ding, K. Xu, S. S. Zhang, K. Amine, G. L. Henriksen, T. R. Jow, *Journal of The Electrochemical Society* **2001**, *148*, A1196.
[61] N. Bjerrum, *Det Kgl. Danske Videnskabernes Selskab.* **1926**.
[62] Y. Marcus, G. Hefter, *Chemical Reviews* **2006**, *106*, 4585.
[63] L. Lehnert, M. Nojabaee, A. Latz, B. Horstmann, *ChemElectroChem* **2024**, *11*.
[64] M. Gouverneur, J. Kopp, L. van Wüllen, M. Schönhoff, *Physical Chemistry Chemical Physics* **2015**, *17*, 30680.
[65] E. Pettersson, I. Furó, P. Stilbs, *Concepts in Magnetic Resonance Part A* **2004**, *22A*, 61.
